# Supplementary material for: State- versus Reaction-Based Information Processing in Biochemical Networks
Source: arXiv:2505.13373 source file (2026-06-17)
Supplement: Supplementary file 1 [file appendix.pdf]

# Supplementary Material

## State- versus Reaction-Based Information Processing in Biochemical Networks

Anne-Lena Moor, Age Tjalma, Manuel Reinhardt,
Pieter Rein ten Wolde, Christoph Zechner

## A. Linear Noise Approximation

In the main text, we describe the dynamics of the system using the Chemical Langevin Equation under the Linear Noise Approximation [1]. In this description, we describe the state of the system with a continuous variable $z(t)$, which evolves in time according to reactions with propensity functions $h_k(z(t))$, $k \in K$, with $K$ being the number of reaction types. Generally, the dependencies of the system's state are non-linear. Hence, the propensity functions are linear only for special cases, such as unimolecular reactions following mass action kinetics. This means that the moments of $z(t)$ can depend on moments of higher order. To address these non-linearities, Van Kampen suggested an approximation method called Linear Noise Approximation [1]. Usually, the Linear Noise Approximation is derived from the Chemical Master Equation [1, 2]. An intuitive derivation can be obtained from the Chemical Langevin Equation directly as suggested in [3] and we will adopt this approach in the following. For $z(t)$ denoting the state of the system in terms of copy numbers, we obtain the concentration

$$\zeta(t) = \frac{z(t)}{\Omega}. \tag{A.1}$$

We further define rescaled propensity functions as $\tilde{h}_k(\zeta(t)) = h_k(z(t))/\Omega$. With this change of variables, we can write the evolution of the system's state in terms of $\zeta(t)$ as

$$\mathrm{d}\zeta(t) = \sum_{k=1}^{K} \left( s_k \tilde{h}_k(\zeta(t))\mathrm{d}t + s_k \sqrt{\frac{\tilde{h}_k(\zeta(t))}{\Omega}} \mathrm{d}w_k(t) \right), \tag{A.2}$$

where $s_k$ the stoichiometric change vector of reaction $k$ and $\mathrm{d}w_k(t) \sim \mathcal{N}(0,1)\sqrt{\mathrm{d}t}$ is the increment of a Wiener process $w_k(t)$ with mean 0 and variance $t$. We then make use of the ansatz $\zeta(t) = \hat{\zeta}(t) + \varepsilon(t)/\sqrt{\Omega}$, where $\hat{\zeta}(t)$ is the macroscopic mean concentration and $\varepsilon(t)$ captures fluctuations around this mean. To facilitate readability, we will drop the dependence of $\tilde{h}$ on $\hat{\zeta}(t)$ and define $\tilde{h}(\hat{\zeta}(t)) \equiv \tilde{h}(t)$. We next insert the ansatz into Eq. (A.2) and perform an expansion for small $1/\sqrt{\Omega}$ such that

$$\begin{aligned} \mathrm{d}\zeta(t) \approx \mathrm{d}\left(\hat{\zeta}(t) + \frac{\varepsilon(t)}{\sqrt{\Omega}}\right) = \sum_{k=1}^{K} \Bigg( s_k \tilde{h}_k(t)\mathrm{d}t + s_k (\nabla \tilde{h}_k(t))^T \frac{\varepsilon(t)}{\sqrt{\Omega}} \mathrm{d}t \\ + s_k \sqrt{\frac{\tilde{h}_k(t)}{\Omega}} \mathrm{d}w_k(t) \Bigg) + \mathcal{O}\left(\frac{1}{\Omega}\right), \end{aligned} \tag{A.3}$$

where $(\nabla \tilde{h}_k)_i = \partial_{\zeta_i} \tilde{h}_k$. Collecting terms of equal order in $1/\sqrt{\Omega}$ yields

$$\mathrm{d}\hat{\zeta}(t) = \sum_{k=1}^{K} s_k \tilde{h}_k(t)\mathrm{d}t \tag{A.4}$$

and

$$\mathrm{d}(\varepsilon(t)) = \sum_{k=1}^{K} s_k \left( (\nabla \tilde{h}_k(t))^T \varepsilon(t)\mathrm{d}t + \sqrt{\tilde{h}_k(t)} \mathrm{d}w_k(t) \right), \tag{A.5}$$

which together constitute the Linear Noise Approximation [4][3]. Note that equation (A.5) can be rewritten into an equivalent form, in which the reaction specific noise terms are summarised to an effective noise term using the identity $\sigma_1 \mathrm{d}w_1(t) + \sigma_2 \mathrm{d}w_2(t) = \sqrt{\sigma_1^2 + \sigma_2^2}\mathrm{d}w(t)$. Then Eq. (A.5) reads

$$\mathrm{d}(\varepsilon(t)) = \sum_{k=1}^{K} s_k (\nabla \tilde{h}_k(t))^T \varepsilon(t)\mathrm{d}t + \mathrm{d}\xi(t), \tag{A.6}$$

where $\mathrm{d}\xi(t)$ is the $M$-dimensional noise vector with entries $\sqrt{\sum_{k=1}^{K} s_{z_i,k}^2 \tilde{h}_k(t)}\mathrm{d}w_{z_i}(t)$, $i \in \{1,...,M\}$ as also defined in the main text. From Eq. (A.5) and Eq. (A.6), we can readily obtain the copy number fluctuations $\delta z(t)$ via $\delta z(t) = \sqrt{\Omega}\varepsilon(t)$. Considering $\tilde{h}_k(\zeta(t)) = h_k(z(t))/\Omega$ and rewriting Eq. (A.5) in matrix notation, Eq. (A.5) corresponds to Eq. (1) in the main text. Note that we restrict our analyses to steady state regimes, such that all time-dependent coefficients in Eq. (A.5) become constant.

## B. Reaction-Based Description of the System

In the previous section, we provided two equivalent ways of describing the system under the Linear Noise Approximation given by Eq. (A.5) and Eq. (A.6). Commonly, Eq. (A.6) is used to describe the system effectively via the superposition of the $M$-dimensional kinetic drift vector

$$\phi(z(t))\mathrm{d}t := \sum_{k=1}^{K} s_k \underbrace{(\nabla h_k(\hat{z}(t)))^T \delta z(t)}_{\lambda_k(z(t))} \mathrm{d}t \tag{B.1}$$

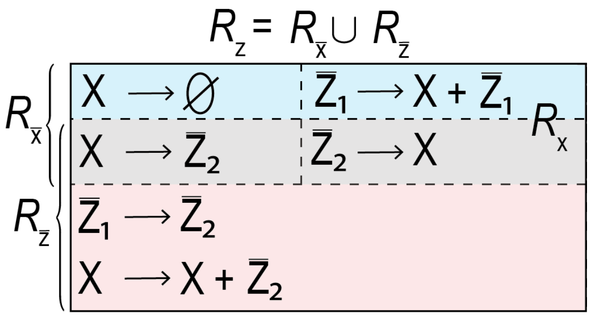


Figure 1: Example network and the corresponding reaction sets. The species X is the observable one, i.e. the species we condition on. The species $\bar{Z}_i$, $i \in \{1,2\}$ denote all other species, i.e. the species that we do not observe. The set $R_{\bar{z}}$ contains all reactions that modify $\bar{z}(t)$. Analogously, the set $R_{\bar{x}}$ contains all reactions that modify $x(t)$. Generally, the intersection $R_{\bar{z}} \cap R_{\bar{x}}$ is not empty. The set $R_x \subseteq R_{\bar{x}}$ contains all reactions that modify $x(t)$ and depend on a species in $\bar{z}(t)$ (reactions on the right of the vertical dashed line). Also in this case, the intersection $R_{\bar{z}} \cap R_x$ is not empty.

and the $M$-dimensional noise vector with entries

$$\mathrm{d}\xi_{z_i}(t) := \sum_{k=1}^{K} s_{z_i,k} \underbrace{\sqrt{h_k(z^*)}}_{\sigma_k} \mathrm{d}w_k(t) = \underbrace{\sqrt{\sum_{k=1}^{K} s_{z_i,k}^2 \sigma_k^2},}_{\sigma_{z_i}\mathrm{d}w_{z_i}(t)} \tag{B.2}$$

where the noise depends on the steady state $z^*$ of the macroscopic mean and hence, is constant. In this sense, the path is defined via the increments of an $M$-dimensional Wiener process with entries

$$\mathrm{d}w_{z_i}(t) = \sigma_{z_i}^{-1}\left(\mathrm{d}(\delta z_i(t)) - \phi_{z_i}(z(t))\mathrm{d}t\right) \tag{B.3}$$

which leads to the state-based description of a path. Here, we introduce a reaction-based description of the path, which collects information about each individual reaction channel. To this end, instead of focusing on copy number increments, $\mathrm{d}(\delta z(t))$ is divided into reaction increments as

$$\mathrm{d}(\delta z(t)) = \sum_{k=1}^{K} \mathrm{d}(\delta z_k(t)) \tag{B.4}$$

with

$$\mathrm{d}(\delta z_k(t)) = s_k \lambda_k(z(t))\mathrm{d}t + s_k \sigma_k \mathrm{d}w_k(t) = s_k \mathrm{d}r_k(t), \tag{B.5}$$

where $\mathrm{d}r_k(t) := \lambda_k(z(t))\mathrm{d}t + \sigma_k \mathrm{d}w_k(t)$ defines the increment of reaction $k$. As a consequence, the path can be defined as $K$ independent increments of Wiener processes

$$\mathrm{d}w_k(t) = \frac{\mathrm{d}r_k(t) - \lambda_k(z(t))\mathrm{d}t}{\sigma_k}. \tag{B.6}$$

In this context, the increment $\mathrm{d}w_k(t)$ defines the fluctuations that are caused by each reaction individually.

## C. Reaction Sets

In this section, we aim to explain the reaction sets used throughout this paper in detail. We restrict ourselves to the sets $R_z, R_{\bar{z}}, R_{\bar{x}}$ and $R_x$ because $R_{\bar{y}}$ and $R_y$ follow the same rules as $R_{\bar{x}}$ and $R_x$. Let $z(t)$ be a vector containing the state of all species at time $t$. The reaction set $R_z$ contains all reactions that modify any species in $z(t)$. Let $x(t) \subseteq z(t)$ be the state of the species we observe. In the main text, we are interested in the conditional expectation value of all species other than X given the history $x_0^t$ of $x(t)$. In this context, $\bar{z}(t) \subseteq z(t)$ denotes the state of all species other than $x(t)$, i.e. the part of $z(t)$ that we do not observe. The subset $R_{\bar{z}} \subseteq R_z$ is the set of all reactions that modify $\bar{z}(t)$. Analogously, the set $R_{\bar{x}} \subseteq R_z$ is the set of all reactions that modify $x(t)$. As $x(t)$ and $\bar{z}(t)$ can change simultaneously, the intersection of these sets is generally not empty, i.e. $R_{\bar{z}} \cap R_{\bar{x}} \neq \emptyset$. With $R_x \subseteq R_{\bar{x}}$, we denote the set of reactions that modify $x(t)$ and whose rate depends on a species in $\bar{z}(t)$, such as the reactions $Z_1 \to X + Z_1$ or $Z_2 \to X$. Because $x(t)$ and $\bar{z}(t)$ can again change simultaneously we have that $R_{\bar{z}} \cap R_x \neq \emptyset$. Fig. 1 illustrates how different reactions are assigned to the various sets.

## D. Derivation of the Reaction-Based Path Mutual Information

In this section we derive the Gaussian path mutual information for reaction-based paths stated in the main text. Generally, the mutual information between two paths $x_0^t, y_0^t \subset z_0^t$ is given by

$$I_t^{XY} = \left\langle \log \frac{\mathrm{d}P^{xy}}{\mathrm{d}(P^x \times P^y)} \right\rangle, \tag{D.1}$$

where $\mathrm{P}^{xy}$ is the joint path measure corresponding to the combined path $\{x_0^t, y_0^t\}$ and $\mathrm{P}^x$ and $\mathrm{P}^y$ are marginal path measures corresponding to the respective paths $x_0^t$ and $y_0^t$. The ratio inside the logarithm of Eq. (D.1) corresponds to a likelihood ratio, formally obtained as a Radon-Nikodym derivative. To calculate this likelihood ratio, we first consider a complete trajectory $z_0^t$ in the reaction-based formalism satisfying Eq. (A.5). We denote by $P^Z$ the measure associated with this process. The Radon-Nikodym derivative between $P^z$ and some reference measure $Q^z$ is given by [5]

$$\frac{\mathrm{d}P^z}{\mathrm{d}Q^z} = \prod_k \exp\left( \int_0^t \frac{\lambda_k(z(s))}{\sigma_k^2} \mathrm{d}r_k(s) - \int_0^t \frac{1}{2} \frac{\lambda_k(z(s))^2}{\sigma_k^2} \mathrm{d}s \right), \tag{D.2}$$

where $\mathrm{d}r_k(t)$ is the reaction increment as defined in Eq. (B.5) and we have chosen $Q^z$ such that all drift terms are zero under $Q^z$. Consider now the marginal path $x_0^t$ associated with measure $P^x$. The likelihood ratio between $P^x$ and some reference measure $Q^x$ is similarly given by

$$\frac{\mathrm{d}P^x}{\mathrm{d}Q^x} = \exp\left( \sum_{k \in R_{\bar{x}}} \int_0^t \frac{\lambda_k^x(s)}{\sigma_k^2} \mathrm{d}r_k(s) - \int_0^t \frac{1}{2} \frac{\lambda_k^x(s)^2}{\sigma_k^2} \mathrm{d}s \right), \tag{D.3}$$

where only reactions are considered which affect $x(t)$ and we have again chosen $Q^x$ to have zero drift terms. Importantly, (D.3) contains modified drift terms [6, 7], which are given by $\lambda_k^x(t) = \langle \lambda_k(z(t)) \mid x_0^t \rangle$, where the expectation is taken with respect to the conditional distribution $P(z(t) = z \mid x_0^t)$. As a consequence of the conditional expectation, the dependency of $\lambda_k^x$ on components other than $x(t)$ is "integrated out" exactly. Analogous considerations apply to likelihood ratios $\mathrm{d}P^y/\mathrm{d}Q^y$ and $\mathrm{d}P^{xy}/\mathrm{d}Q^{xy}$. The likelihood ratio between the marginal measures $P^{xy}$ and $P^x \times P^y$ is then given by

$$\begin{aligned}\frac{\mathrm{d}P^{xy}}{\mathrm{d}(P^x \times P^y)} =& \exp\Big( \sum_{k \in R_{\bar{x}}} \int_0^t \frac{\lambda_k^{xy}(s) - \lambda_k^x(s)}{\sigma_k^2} \mathrm{d}r_k(s) - \frac{1}{2} \int_0^t \frac{\lambda_k^{xy}(s)^2 - \lambda_k^x(s)^2}{\sigma_k^2} \mathrm{d}s \\ &+ \sum_{k \in R_{\bar{y}}} \int_0^t \frac{\lambda_k^{xy}(s) - \lambda_k^y(s)}{\sigma_k^2} \mathrm{d}r_k(s) - \frac{1}{2} \int_0^t \frac{\lambda_k^{xy}(s)^2 - \lambda_k^y(s)^2}{\sigma_k^2} \mathrm{d}s \Big),\end{aligned} \tag{D.4}$$

where the respective reference measures have canceled out. Inserting Eq. (D.4) into Eq. (D.1) leads to

$$\begin{aligned}I_t^{xy} =& \Big\langle -\frac{1}{2} \int_0^t \left( \sum_{k \in R_{\bar{x}}} \frac{\lambda_k^{xy}(s)^2 - \lambda_k^x(s)^2}{\sigma_k^2} + \sum_{k \in R_{\bar{y}}} \frac{\lambda_k^{xy}(s)^2 - \lambda_k^y(s)^2}{\sigma_k^2} \right) \mathrm{d}s \\ &+ \int_0^t \left( \sum_{k \in R_{\bar{x}}} \frac{\lambda_k^{xy}(s) - \lambda_k^x(s)}{\sigma_k^2} + \sum_{k \in R_{\bar{y}}} \frac{\lambda_k^{xy}(s) - \lambda_k^y(s)}{\sigma_k^2} \right) \mathrm{d}r_k(s) \Big\rangle.\end{aligned} \tag{D.5}$$

Next, we replace the increment $\mathrm{d}r_k(t) = \lambda_k^{xy}(t)\mathrm{d}t + \sigma_k \mathrm{d}w_k(t)$ to simplify the equation. Considering that $\langle \lambda_k^{xy}(t) \lambda_k^x(t) \rangle = \langle \langle \lambda_k^{xy}(t) \mid x_0^t \rangle \lambda_k^x(t) \rangle = \langle \lambda_k^x(t)^2 \rangle$, the cross-terms vanish and we obtain

$$\begin{aligned}I_t^{xy} =& \Big\langle \frac{1}{2} \int_0^t \left( \sum_{k \in R_{\bar{x}}} \frac{\lambda_k^{xy}(s)^2 - \lambda_k^x(s)^2}{\sigma_k^2} + \sum_{k \in R_{\bar{y}}} \frac{\lambda_k^{xy}(s)^2 - \lambda_k^y(s)^2}{\sigma_k^2} \right) \mathrm{d}s \\ &+ \int_0^t \left( \sum_{k \in R_{\bar{x}}} \frac{\lambda_k^{xy}(s) - \lambda_k^x(s)}{\sigma_k} + \sum_{k \in R_{\bar{y}}} \frac{\lambda_k^{xy}(s) - \lambda_k^y(s)}{\sigma_k} \right) \mathrm{d}w_k(s) \Big\rangle \\ =& \left\langle \frac{1}{2} \int_0^t \left( \sum_{k \in R_{\bar{x}}} \frac{\lambda_k^{xy}(s)^2 - \lambda_k^x(s)^2}{\sigma_k^2} + \sum_{k \in R_{\bar{y}}} \frac{\lambda_k^{xy}(s)^2 - \lambda_k^y(s)^2}{\sigma_k^2} \right) \mathrm{d}s \right\rangle,\end{aligned} \tag{D.6}$$

where the second equality results from the fact that $\langle \mathrm{d}w_k(t) \rangle = 0$ for all $k \in R_z$. This expression can be simplified further because only reactions in $R_{\bar{x}}$ have to be considered whose rate depends on species other than X. All other reactions will cancel as for these reactions $\lambda_k^{xy}(t) = \lambda_k^x(t)$. For instance, a reaction with drift $\alpha x(t)$ will cancel as this results in $\lambda_k^{xy}(t) = \alpha \langle x(t) \mid x_0^t, y_0^t \rangle = \alpha x(t) = \alpha \langle x(t) \mid x_0^t \rangle = \lambda_k^x(t)$, whereas a reaction with drift $\alpha \bar{z}_i(t)$ would remain as $\lambda_k^{xy}(t) = \alpha \langle \bar{z}_i(t) \mid x_0^t, y_0^t \rangle \neq \alpha \langle \bar{z}_i(t) \mid x_0^t \rangle = \lambda_k^x(t)$ in general. Equivalent considerations hold for $y(t)$. The sets of reactions that affect X and Y but depend on species other than X or Y are denoted as $R_x$ and $R_y$, respectively. Exchanging the order of the integral and expectation results in

$$I_t^{xy} = \frac{1}{2} \int_0^t \sum_{k \in R_x} \frac{\langle \lambda_k^{xy}(s)^2 \rangle - \langle \lambda_k^x(s)^2 \rangle}{\sigma_k^2} + \sum_{k \in R_y} \frac{\langle \lambda_k^{xy}(s)^2 \rangle - \langle \lambda_k^y(s)^2 \rangle}{\sigma_k^2} \mathrm{d}s. \tag{D.7}$$

Next, we can rewrite the second moments into variances. It follows from the law of total expectation that $\langle \lambda_k^{xy}(t) \rangle = \langle \lambda_k^x(t) \rangle$ for $k \in R_x$ and $\langle \lambda_k^{xy}(t) \rangle = \langle \lambda_k^y(t) \rangle$ for $k \in R_y$. Hence, Eq. (D.7) is equivalent to

$$\begin{aligned} I_t^{xy} &= \frac{1}{2}\int_0^t \sum_{k\in R_x} \frac{\langle \lambda_k^{xy}(s)^2 \rangle - \langle \lambda_k^{xy}(s) \rangle^2 - \langle \lambda_k^x(s)^2 \rangle + \langle \lambda_k^x(s) \rangle^2}{\sigma_k^2} \\ &\quad + \sum_{k\in R_y} \frac{\langle \lambda_k^{xy}(s)^2 \rangle - \langle \lambda_k^{xy}(s) \rangle^2 - \langle \lambda_k^y(s)^2 \rangle + \langle \lambda_k^y(s) \rangle^2}{\sigma_k^2} \mathrm{d}s \\ &= \frac{1}{2}\int_0^t \sum_{k\in R_x} \frac{\mathrm{Var}\left[\lambda_k^{xy}(s)\right] - \mathrm{Var}\left[\lambda_k^x(s)\right]}{\sigma_k^2} + \sum_{k\in R_y} \frac{\mathrm{Var}\left[\lambda_k^{xy}(s)\right] - \mathrm{Var}\left[\lambda_k^y(s)\right]}{\sigma_k^2} \mathrm{d}s. \end{aligned} \tag{D.8}$$

Finally, the latter can be brought into a simpler form by rewriting the variances of the conditional expectations into expected conditional variances as those are more convenient to calculate in practice. According to the law of total variance, it follows

$$\begin{aligned} I_t^{xy} =& \frac{1}{2}\int_0^t \sum_{k\in R_x} \frac{\left\langle \mathrm{Var}\left[\lambda_k(z(s)) \mid x_0^t\right] \right\rangle - \left\langle \mathrm{Var}\left[\lambda_k(z(s)) \mid x_0^t, y_0^t\right] \right\rangle}{\sigma_k^2} \\ &+ \sum_{k\in R_y} \frac{\left\langle \mathrm{Var}\left[\lambda_k(z(s)) \mid y_0^t\right] \right\rangle - \left\langle \mathrm{Var}\left[\lambda_k(z(s)) \mid x_0^t, y_0^t\right] \right\rangle}{\sigma_k^2} \mathrm{d}s. \end{aligned} \tag{D.9}$$

Interestingly, the first and second line in Eq. (D.9) reflect the respective transfer entropies $H_t^{y\to x}$ and $H_t^{x\to y}$ [8]. Note that Eq. (D.9) is not valid for systems involving reactions where (a) the species X and Y are modified simultaneously and (b) the corresponding rate function depends on both $x(t)$ and $y(t)$. An example of such reaction is $\mathrm{Y} + \mathrm{X} \to \emptyset$.

## E. Derivation of the State-based Path Mutual Information

Similarly to the reaction-based path mutual information, we can derive a state-based form using Eq. (D.1). We follow the same procedure, with the only difference that we now consider paths defined through state increments rather than reaction increments. For the sake of illustration, let us again consider the marginal path $\tilde{x}_0^t$ and associated measure $\tilde{P}^x$, where the tilde indicates that we are working with the state-based formalism. The likelihood-ratio between $\tilde{P}^x$ and a zero-drift reference measure $\tilde{Q}^x$ is now given by

$$\frac{\mathrm{d}\tilde{P}^x}{\mathrm{d}\tilde{Q}^x} = \exp\left(\int_0^t \frac{\phi_x^x(s)}{\sigma_x^2}\mathrm{d}x(s) - \int_0^t \frac{1}{2}\frac{\phi_x^x(s)^2}{\sigma_x^2}\mathrm{d}s\right), \tag{E.1}$$

where the original drifts terms $\phi^x(t)$ have been replaced by $\phi_x^x(t) = \langle \phi_x(z(t)) \mid \tilde{x}_0^t \rangle$. Equivalent considerations hold for $y(t) \subset z(t)$ and $(x(t), y(t)) \subset z(t)$ such that we obtain

$$\begin{aligned} \frac{\mathrm{d}\tilde{P}^{xy}}{\mathrm{d}(\tilde{P}^x \times \tilde{P}^y)} =& \exp\Bigg(\int_0^t \frac{\phi_x^{xy}(s) - \phi_x^x(s)}{\sigma_x^2}\mathrm{d}x(s) - \frac{1}{2}\int_0^t \frac{\phi_x^{xy}(s)^2 - \phi_x^x(s)^2}{\sigma_x^2}\mathrm{d}s \\ &+ \int_0^t \frac{\phi_y^{xy}(s) - \phi_y^y(s)}{\sigma_y^2}\mathrm{d}y(s) - \frac{1}{2}\int_0^t \frac{\phi_y^{xy}(s)^2 - \phi_y^y(s)^2}{\sigma_y^2}\mathrm{d}s\Bigg), \end{aligned} \tag{E.2}$$

with $\phi_y^y(t) = \langle \phi_y(z(t)) \mid \tilde{y}_0^t \rangle$ and $\phi_x^{xy}(t) = \langle \phi_x(z(t)) \mid \tilde{x}_0^t, \tilde{y}_0^t \rangle$ and correspondingly $\phi_y^{xy}(t) = \langle \phi_y(z(t)) \mid \tilde{x}_0^t, \tilde{y}_0^t \rangle$. Performing calculations analogously to the ones for obtaining Eq. (D.8) and decomposing the drift terms into reaction-specific contributions, we obtain for the state-based path mutual information

$$\begin{aligned} \tilde{I}_t^{xy} =& \frac{1}{2}\int_0^t \sum_{k\in R_x} \frac{s_{x,k}^2}{\sigma_x^2}\left(\left\langle \mathrm{Var}\left[\lambda_k(z(s)) \mid \tilde{x}_0^t\right] \right\rangle - \left\langle \mathrm{Var}\left[\lambda_k(z(s)) \mid \tilde{x}_0^t, \tilde{y}_0^t\right] \right\rangle\right) \\ &+ \sum_{k\in R_y} \left(\frac{s_{y,k}^2}{\sigma_y^2}\left\langle \mathrm{Var}\left[\lambda_k(z(s)) \mid \tilde{y}_0^t\right] \right\rangle - \left\langle \mathrm{Var}\left[\lambda_k(z(s)) \mid \tilde{x}_0^t, \tilde{y}_0^t\right] \right\rangle\right)\mathrm{d}s \end{aligned} \tag{E.3}$$

Comparing Eq. (E.3) to Eq. (D.9), one can see that the main difference in the structure of these equations lies in the denominators, which are given by the noise magnitude in the respective formalism. In the reaction-based formalism, we obtain one noise magnitude $\sigma_k$ per each reaction channel, while in the concentration-based formalism, all reaction-specific noise contributions are summarized into a single effective noise magnitude, i.e. $\sigma_x = \sqrt{\sum_{k\in R_{\tilde{x}}} s_{x,k}^2 \sigma_k^2}$.

The mutual information between state-based Gaussian processes has been studied previously, for instance in [9], where similar results have been obtained. The way we derived Eq. (E.3) is specific to chemical reaction networks – the dynamics of which are linearised using the Linear Noise Approximation.

Eq. (E.3) is closely connected to the result obtained by Tostevin *et al.* in [12]. For reaction networks in which $x(t)$ (or $y(t)$) do not change simultaneously with a species $\bar{\mathrm{Z}}$, such as motif a in Table 1 in the main text, these methods provide the

same result. In these situations, the stochastic Wiener increments of $x(t)$ (or $y(t)$) and $\bar{z}(t)$ are uncorrelated. In the presence of correlated increments (e.g., motif b in Table 1), the method of Tostevin *et al.* can result in diverging information rates (see [13] for in-depth discussion). These scenarios are not within the scope of Eq. (E.3), since we have excluded networks where $x(t)$ (or $y(t)$) and $\bar{z}(t)$ change simultaneously in our derivation. Extending our analysis to include such situations, will be an interesting subject for the future.

## F. Derivation of the Reaction-Based Filtering Equation

The aim of this section is to derive Eq. (5) of the main text, a filtering equation for a system obeying reaction-based Gaussian dynamics. In contrast to the state-based formalism, Eq. (5) applies also to cases where $x(t)$ (or $y(t)$) changes simultaneously with $\bar{z}(t)$. As a consequence of this, the considered system is not compatible with a standard Kalman-Bucy filter [14, 15], because some of the noise terms enter the dynamics of both $x(t)$ and $\bar{z}(t)$. In the following, we derive a filtering equation for this scenario, following standard procedures [16, 15].

In the reaction-based formalism, we distinguish between individual reactions as discussed in Section B. Therefore, we can write the dynamics of the state of the system $z(t)$ as

$$\mathrm{d}\left(\delta z(t)\right) = \sum_{k=1}^{K} \mathrm{d}z_k(t) = s_k \lambda_k(z(t))\mathrm{d}t + s_k \sigma_k \mathrm{d}w_k(t) \tag{F.1}$$

where $\mathrm{d}z_k(t)$ defines the increment of $\delta z(t)$ corresponding to reaction $k$, and $\lambda_k$ and $\sigma_k$ define the drift and noise contributions to the increment according to the Linear Noise Approximation (see Eq. (B.1) and Eq. (B.2)). For our purpose, we divide the system's state $z(t)$ into two parts $x(t)$ and $\bar{z}(t)$ where $x(t)$ corresponds to the *observable* part of the system (i.e., the part that we condition on) and $\bar{z}(t)$ collects the *hidden* components of the system (i.e., the components that are reconstructed from the observation). We aim to derive a differential equation for $\pi^x(\bar{z},t) = p(\bar{z}(t) \mid x_0^t)$.

To this end, we first derive a differential equation for the conditional expectation of some generic function $g(\bar{z}(t))$ because statistics and probabilities can be expressed as expectations over appropriately chosen functions. However, since the conditional expectation is difficult to calculate, we perform a change of measure and proceed by calculating the conditional expectation value under the auxiliary measure $Q^z$ instead of $P^z$. As the result is independent of the particular choice of $Q^z$, we can choose it in a way that simplifies the calculation. The probability measure can be changed according to

$$\langle g(\bar{z}(t)) \mid x_0^t \rangle = \frac{\langle g(\bar{z}(t)) l(\bar{z}_0^t, x_0^t) \mid x_0^t \rangle_{Q^z}}{\langle l(\bar{z}_0^t, x_0^t) \mid x_0^t \rangle_{Q^z}} \tag{F.2}$$

where $l(\bar{z}_0^t, x_0^t) = \mathrm{d}P^z/\mathrm{d}Q^z$ is a Radon-Nikodym derivative, and $\bar{z}_0^t$ and $x_0^t$ are complete trajectories of $\bar{z}(t)$ and $x(t)$, respectively [16][15]. For deriving the filtering equation we can use stochastic calculus to derive differential equations for the respective terms in (F.2) and subsequently take the expectation.

We first consider the differential of $g(\bar{z}(t))$, which according to Ito's lemma can be written as

$$\mathrm{d}g(\bar{z}(t)) = \sum_{k \in R_{\bar{z}}} \Big( s_{\bar{z},k}^T \lambda_k(\bar{z}(t),x(t)) \partial_{\bar{z}} g(\bar{z}(t))\mathrm{d}t + \sum_{i=1}^{M_{\bar{z}}} \frac{1}{2} s_{\bar{z}_i,k}^2 \sigma_k^2 \partial_{\bar{z}_i}^2 g(\bar{z}(t))\mathrm{d}t + s_{\bar{z},k}^T \sigma_k \partial_{\bar{z}} g(\bar{z}(t))\mathrm{d}w_k(t) \Big) \tag{F.3}$$

where $R_{\bar{z}}$ describes the set of reactions that modify $\bar{z}(t)$ and $M_{\bar{z}}$ denotes the number of species in $\bar{\mathrm{Z}}$. Note, that $s_{\bar{z},k}\lambda_k$ describes the drift under the measure $P^z$ with $s_{\bar{z},k}$ being the part of the stoichiometric change vector of reaction $k$ acting on $\bar{z}(t)$. Under the measure $Q^z$, the drift is denoted by $s_{\bar{z},k}\tilde{\lambda}_k$ whereas the noise magnitude $\sigma_k$ is the same as under $P^z$. According to Eq. (F.2) we can write the Radon-Nikodym derivative as

$$\begin{aligned} l(\bar{z}_0^t, x_0^t) = \exp\Big( &\sum_{k \in R_{\bar{z}} \setminus R_{\bar{x}}} \int_0^t \frac{\lambda_k(\bar{z}(s),x(s)) - \tilde{\lambda}_k(\bar{z}(s),x(s))}{\sigma_k} \mathrm{d}w_k(s) + \frac{1}{2}\int_0^t \frac{\Big(\lambda_k(\bar{z}(s),x(s)) - \tilde{\lambda}_k(\bar{z}(s),x(s))\Big)^2}{\sigma_k^2} \mathrm{d}s \\ &+ \sum_{k \in R_{\bar{x}}} \int_0^t \frac{\lambda_k(\bar{z}(s),x(s)) - \tilde{\lambda}_k(\bar{z}(s),x(s))}{\sigma_k} \mathrm{d}w_k(s) + \frac{1}{2}\int_0^t \frac{\Big(\lambda_k(\bar{z}(s),x(s)) - \tilde{\lambda}_k(\bar{z}(s),x(s))\Big)^2}{\sigma_k^2} \mathrm{d}s \Big). \end{aligned} \tag{F.4}$$

where $R_{\bar{x}}$ denotes the set of reactions that modify $x(t)$. Note that we distinguish between reactions $R_{\bar{x}}$ that modify $x(t)$ and reactions $R_{\bar{z}} \setminus R_{\bar{x}}$ that modify species other than $x(t)$. We now choose the auxiliary measure $Q^z$ to simplify the calculations. In particular, we choose $Q^z$ such that $\tilde{\lambda}_k = \lambda_k$ for $k \in R_{\bar{z}} \setminus R_{\bar{x}}$, that is, reactions that do not affect $x(t)$. For reactions that do affect $x(t)$, we choose $\tilde{\lambda}_k = 0$. With that particular choice, many terms cancel out so that we can write Eq. (F.4) as

$$l(\bar{z}_0^t, x_0^t) = \exp\Big( \sum_{k \in R_{\bar{x}}} \frac{1}{2}\int_0^t \frac{\lambda_k(\bar{z}(s),x(s))^2}{\sigma_k^2}\mathrm{d}s + \int_0^t \frac{\lambda_k(\bar{z}(s),x(s))}{\sigma_k}\mathrm{d}w_k(s) \Big). \tag{F.5}$$

Using Ito's lemma, we obtain for the differential of $l(\bar{z}_0^t, x_0^t)$

$$\mathrm{d}l(\bar{z}_0^t, x_0^t) = l(\bar{z}_0^t, x_0^t) \Big[ \sum_{k \in R_{\bar{x}}} \frac{\lambda_k(\bar{z}(t),x(t))^2}{\sigma_k^2}\mathrm{d}t + \frac{\lambda_k(\bar{z}(t),x(t))}{\sigma_k}\mathrm{d}w_k(t) \Big]. \tag{F.6}$$

Having obtained the differential of $l(\bar{z}_0^t, x_0^t)$, we can apply Ito's lemma to the product $g(\bar{z}(t))l(\bar{z}_0^t, x_0^t)$ as

$$\begin{aligned}\mathrm{d}\big[g(\bar{z}(t))l(\bar{z}_0^t,x_0^t)\big] =& l(\bar{z}_0^t,x_0^t)\Big[\sum_{k\in R_{\bar{z}}}\Big(s_{\bar{z},k}^T\partial_{\bar{z}}g(\bar{z}(t))\lambda_k(\bar{z}(t),x(t))\mathrm{d}t+\sum_{i=1}^{M_{\bar{z}}}\frac{1}{2}s_{\bar{z}_i,k}^2\sigma_k^2\partial_{\bar{z}_i}^2 g(\bar{z}(t))\mathrm{d}t+s_{\bar{z},k}^T\sigma_k\partial_{\bar{z}}g(\bar{z}(t))\mathrm{d}w_k(t)\Big)\Big]\\&+g(\bar{z}(t))l(\bar{z}_0^t,x_0^t)\sum_{k\in R_{\bar{x}}}\frac{\lambda_k(\bar{z}(t),x(t))}{\sigma_k^2}\big(\lambda_k(\bar{z}(t),x(t))\mathrm{d}t+\sigma_k\mathrm{d}w_k(t)\big)\\&+\sum_{k\in R_{\bar{z}}\cap R_{\bar{x}}}s_{\bar{z},k}^T\lambda_k(\bar{z}(t),x(t))\partial_{\bar{z}}g(\bar{z}(t))l(\bar{z}_0^t,x_0^t)\mathrm{d}t,\end{aligned} \tag{F.7}$$

where the last term results from the fact that $\mathrm{d}g(\bar{z}(t))$ and $\mathrm{d}l(\bar{z}_0^t,x_0^t)$ have common noise terms, i.e. $\mathrm{d}g(\bar{z}(t))\mathrm{d}l(\bar{z}_0^t,x_0^t)\neq 0$ as $R_{\bar{z}}\cap R_{\bar{x}}\neq\emptyset$. Before we evaluate expectations under $Q^z$, we substitute $\mathrm{d}w_k(t)=\sigma_k^{-1}(\mathrm{d}r_k(t)-\lambda_k(\bar{z}(t),x(t)))\mathrm{d}t$, because the decomposition of the reaction increments into $\lambda_k\mathrm{d}t$ and a Wiener increment is specific to $P^z$. In particular, we obtain

$$\begin{aligned}\mathrm{d}\big[g(\bar{z}(t))l(\bar{z}_0^t,x_0^t)\big] =& l(\bar{z}_0^t,x_0^t)\Big[\sum_{k\in R_{\bar{z}}}\Big(s_{\bar{z},k}^T\partial_{\bar{z}}g(\bar{z}(t))\mathrm{d}r_k(t)+\sum_{i=1}^{M_{\bar{z}}}\frac{1}{2}s_{\bar{z}_i,k}^2\sigma_k^2\partial_{\bar{z}_i}^2 g(\bar{z}(t))\mathrm{d}t\Big)\Big]\\&+g(\bar{z}(t))l(\bar{z}_0^t,x_0^t)\sum_{k\in R_{\bar{x}}}\frac{\lambda_k(\bar{z}(t),x(t))}{\sigma_k^2}\mathrm{d}r_k(t)\big)+\sum_{k\in R_{\bar{z}}\cap R_{\bar{x}}}s_{\bar{z},k}^T\lambda_k(\bar{z}(t),x(t))\partial_{\bar{z}}g(\bar{z}(t))l(\bar{z}_0^t,x_0^t)\mathrm{d}t.\end{aligned} \tag{F.8}$$

Defining the generator

$$\mathscr{A}^*g(\bar{z}(t))\mathrm{d}t:=\sum_{i=1}^{M_{\bar{z}}}\sum_{k\in R_{\bar{z}_i}}\Big(\partial_{\bar{z}_i}g(\bar{z}(t))s_{\bar{z}_i,k}\lambda_k(\bar{z}(t),x(t))\mathrm{d}t+\frac{1}{2}s_{\bar{z}_i,k}^2\sigma_k^2\partial_{\bar{z}_i}^2g(\bar{z}(t))\mathrm{d}t\Big) \tag{F.9}$$

and calculating the conditional expectation with respect to $Q^z$, we can write

$$\begin{aligned}\mathrm{d}\big\langle g(\bar{z}(t))l(\bar{z}_0^t,x_0^t)\mid x_0^t\big\rangle_{Q^z} =& \big\langle l(\bar{z}_0^t,x_0^t)\mathscr{A}^*g(\bar{z}(t))\mid x_0^t\big\rangle_{Q^z}\mathrm{d}t+\sum_{k\in R_{\bar{z}}}s_{\bar{z},k}^T\Big\langle l(\bar{z}_0^t,x_0^t)\partial_{\bar{z}}g(\bar{z}(t))\left(\mathrm{d}r_k(t)-\lambda_k(\bar{z}(t),x(t))\mathrm{d}t\right)\Big|x_0^t\Big\rangle_{Q^z}\\&+\sum_{k\in R_{\bar{x}}}\frac{\langle g(\bar{z}(t))l(\bar{z}_0^t,x_0^t)\lambda_k(\bar{z}(t),x(t))\mid x_0^t\rangle_{Q^z}}{\sigma_k^2}\mathrm{d}r_k(t)+\sum_{k\in R_{\bar{z}}\cap R_{\bar{x}}}s_{\bar{z},k}^T\langle l(\bar{z}_0^t,x_0^t)\partial_{\bar{z}}g(\bar{z}(t))\mid x_0^t\rangle_{Q^z}\mathrm{d}r_k(t),\end{aligned} \tag{F.10}$$

where the reaction increments $\mathrm{d}r_k(t)$ are "observed" and can thus be pulled out of the expectation. To obtain an equation for the conditional distribution, we now set $g(\bar{z}(t)):=\delta(\bar{z}-\bar{z}(t))$ such that

$$\pi^x(\bar{z},t)=\langle\delta(\bar{z}-\bar{z}(t))\mid x_0^t\rangle=\frac{\langle\delta(\bar{z}-\bar{z}(t))l(\bar{z}_0^t,x_0^t)\mid x_0^t\rangle_{Q^z}}{\langle l(\bar{z}_0^t,x_0^t)\mid x_0^t\rangle_{Q^z}}. \tag{F.11}$$

Note that the denominator in Eq. (F.11) acts purely as normalisation constant as it does not depend on $\bar{z}$. Defining $\tilde{\pi}^x(\bar{z},t):=\langle\delta(\bar{z}-\bar{z}(t))l(\bar{z}_0^t,x_0^t)\mid x_0^t\rangle_{Q^z}$ as an unnormalised distribution and changing measure back to $P^z$, we can use Eq. (F.10) to obtain

$$\mathrm{d}\tilde{\pi}^x(\bar{z},t)=\mathscr{A}\tilde{\pi}^x(\bar{z},t)\mathrm{d}t+\tilde{\pi}^x(\bar{z},t)\sum_{k\in R_{\bar{x}}}\frac{\lambda_k(\bar{z},x(t))}{\sigma_k^2}\mathrm{d}r_k(t)-\sum_{k\in R_{\bar{z}}\cap R_{\bar{x}}}s_{\bar{z},k}^T\partial_{\bar{z}}\tilde{\pi}^x(\bar{z},t)\mathrm{d}r_k(t), \tag{F.12}$$

where we have used integration by parts and the fact that the Fokker-Planck operator $\mathscr{A}$ is the adjoint of the generator $\mathscr{A}^*$. Note that the second term on the right-hand side of Eq. (F.10) is zero in expectation because $\mathrm{d}r_k(t)-\lambda_k(\bar{z}(t),x(t))\mathrm{d}t$ is a Wiener increment under $P^z$. Eq. (F.12) can be understood as a Zakai equation for reaction-based processes [15]. The main difference to the canonical form of the Zakai equation is that Eq. (F.12) contains additional transport terms, because $\bar{z}(t)$ and $x(t)$ have common noise terms. Note that we have calculated a conditional expectation over components $\bar{z}(t)$ such that the reaction increments are now *marginalised*, i.e,. $\mathrm{d}r_k(t)=\lambda_k^x(t)\mathrm{d}t+\sigma_k\mathrm{d}w_k(t)$ with $\lambda_k^x(t)=\langle\lambda_k(\bar{z}(t),x(t))\mid x_0^t\rangle$ [6, 7].

In order to obtain a normalised filtering equation, we use $\pi^x(\bar{z},t)=\tilde{\pi}^x(\bar{z},t)/C(t)$ with $C(t)=\int\tilde{\pi}^x(\bar{z},t)\mathrm{d}\bar{z}$. By the product rule for Ito processes, we obtain for the change of the normalized distribution

$$\mathrm{d}\frac{\tilde{\pi}^x(\bar{z},t)}{C(t)}=\frac{1}{C(t)}\mathrm{d}\tilde{\pi}^x(\bar{z},t)+\tilde{\pi}^x(\bar{z},t)\mathrm{d}\frac{1}{C(t)}+\mathrm{d}\frac{1}{C(t)}\mathrm{d}\tilde{\pi}^x(\bar{z},t). \tag{F.13}$$

The first term is just (F.12) rescaled by $C(t)$. To calculate the second term, we first calculate $\mathrm{d}C(t)$, which is obtained by integrating (F.12) over $\bar{z}$, i.e.,

$$\mathrm{d}\int\tilde{\pi}^x(\bar{z},t)\mathrm{d}\bar{z}=\sum_{k\in R_{\bar{x}}}\frac{\int\lambda_k(\bar{z},x(t))\tilde{\pi}^x(\bar{z},t)\mathrm{d}\bar{z}}{\sigma_k^2}\mathrm{d}r_k(t), \tag{F.14}$$

where only the second term in Eq. (F.12) contributes a non-zero flux. Using once more Ito's chain rule gives

$$\tilde{\pi}^x(\bar{z},t)\mathrm{d}\frac{1}{C(t)} = -\pi^x(\bar{z},t)\left(\sum_{k\in R_{\bar{x}}}\frac{\langle\lambda_k(\bar{z}(t),x(t))\mid x_0^t\rangle}{\sigma_k^2}\mathrm{d}r_k(t) - \frac{\langle\lambda_k(\bar{z}(t),x(t))\mid x_0^t\rangle^2}{\sigma_k^2}\mathrm{d}t\right), \tag{F.15}$$

where we have substituted $\tilde{\pi}^x(\bar{z},t)/C(t) = \pi^x(\bar{z},t)$ and $\int \lambda_k(\bar{z},x(t))\tilde{\pi}^x(\bar{z},t)/C(t)\mathrm{d}\bar{z} = \langle\lambda_k(\bar{z}(t),x(t))\mid x_0^t\rangle$. The third term is given by

$$\mathrm{d}\frac{1}{C(t)}\mathrm{d}\tilde{\pi}^x(\bar{z},t) = -\pi^x(\bar{z},t)\sum_{k\in R_{\bar{x}}}\frac{\langle\lambda_k(\bar{z}(t),x(t))\mid x_0^t\rangle\lambda_k(\bar{z}(t),x(t))}{\sigma_k^2}\mathrm{d}t + \sum_{k\in R_{\bar{z}}\cap R_{\bar{x}}}\frac{\langle\lambda_k(\bar{z}(t),x(t))\mid x_0^t\rangle s_{\bar{z},k}^T\partial_{\bar{z}}\pi^x(\bar{z},t)}{\sigma_k^2}\mathrm{d}t. \tag{F.16}$$

Adding up all three contributions and rearranging terms leads to the normalised filtering equation

$$\mathrm{d}\pi^x(\bar{z},t) = \mathscr{A}\pi^x(\bar{z},t)\mathrm{d}t + \pi^x(\bar{z},t)\sum_{k\in R_{\bar{x}}}\frac{\lambda_k(\bar{z},x(t)) - \langle\lambda_k(\bar{z}(t),x(t))\mid x_0^t\rangle}{\sigma_k}\mathrm{d}w_k(t) - \sum_{k\in R_{\bar{z}}\cap R_{\bar{x}}} s_{\bar{z},k}^T\sigma_k\partial_{\bar{z}}\tilde{\pi}^x(\bar{z},t)\mathrm{d}w_k(t), \tag{F.17}$$

where we have replaced $\mathrm{d}w_k = \sigma_k^{-1}(\mathrm{d}r_k(t) - \langle\lambda_k(\bar{z}(t),x(t))\mid x_0^t\rangle\mathrm{d}t)$. Realising that $\lambda_k(\bar{z}(t),x(t)) - \langle\lambda_k(\bar{z}(t),x(t))\mid x_0^t\rangle = 0$ for all reactions without $\bar{z}(t)$ in their propensity function, i.e. all reactions except $R_x \subseteq R_{\bar{x}}$, leads to Eq. (5) in the main text. Eq. (F.17) can be understood as a Kushner-Stratonovich equation for reaction-based processes, analogously to the unnormalised Zakai equation from Eq. (F.12).

## G. Derivation of the Covariance Equation

The Gaussian path mutual information given by Eq. (D.9) (Eq. (4), main text) depends only on the expected conditional variances of the propensity functions that directly contribute to the information transfer. For linear propensities, such as those obtained by the Linear Noise Approximation or unimolecular reactions, this results in a dependence on the expected conditional covariances of the chemical species' abundance. For this reason, we derive a general covariance equation for our kind of system as given by Eq. (6) in the main text.

Generally, the expected conditional covariance of two species $\bar{Z}_i$, $\bar{Z}_j$ given the history of $x(t)$ is given by

$$\langle\mathrm{Cov}[\bar{z}_i(t),\bar{z}_j(t)\mid x_0^t]\rangle = \big\langle\langle\bar{z}_i(t)\bar{z}_j(t)\mid x_0^t\rangle - \langle\bar{z}_i(t)\mid x_0^t\rangle\langle\bar{z}_j(t)\mid x_0^t\rangle\big\rangle. \tag{G.1}$$

The respective conditional moments can be obtained using Eq. (F.17). Multiplying Eq. (F.17) with $\bar{z}_i$ and integrating over all $\bar{z}$ leads to the general form of the first conditional moment of a species $\bar{Z}_i$ as

$$\begin{aligned}\mathrm{d}\langle\bar{z}_i(t)\mid x_0^t\rangle = &\int_{\bar{z}}\Big[\sum_{k\in R_{\bar{z}_i}} -\partial_{\bar{z}_i}\big(\bar{z}_i s_{\bar{z}_i,k}\lambda_k(\bar{z},x(t))\pi^x(\bar{z},t)\big)\mathrm{d}t + \frac{1}{2}s_{\bar{z}_i,k}^2\sigma_k^2\partial_{\bar{z}_i}^2\big(\bar{z}_i\pi^x(\bar{z},t)\big)\mathrm{d}t \\ &+ \sum_{k\in R_{\bar{x}}}\frac{\bar{z}_i\left(\lambda_k(\bar{z},x(t)) - \langle\lambda_k(\bar{z}(t),x(t)\mid x_0^t\rangle\right)}{s_{\bar{z}_i,k}\sigma_k}\pi^x(\bar{z},t)\mathrm{d}w_k(t) - \sum_{k\in R_{\bar{z}_i}\cap R_{\bar{x}}}\sigma_{k,i}\partial_{\bar{z}_i}\big(\bar{z}_i\pi^x(\bar{z},t)\big)\mathrm{d}w_k(t)\Big]\mathrm{d}\bar{z} \\ = &\sum_{k\in R_{\bar{z}_i}} s_{\bar{z}_i,k}\langle\lambda_k(\bar{z}(t),x(t))\mid x_0^t\rangle\mathrm{d}t + \sum_{k\in R_{\bar{x}}}\frac{\langle\bar{z}_i(t)\lambda_k(\bar{z}(t),x(t))\mid x_0^t\rangle}{\sigma_k} - \frac{\langle\bar{z}_i(t)\mid x_0^t\rangle\langle\lambda_k(\bar{z}(t),x(t))\mid x_0^t\rangle}{\sigma_k}\mathrm{d}w_k(t) \\ &+ \sum_{k\in R_{\bar{z}_i}\cap R_{\bar{x}}} s_{\bar{z}_i,k}\sigma_k\mathrm{d}w_k(t),\end{aligned} \tag{G.2}$$

where the integrals containing a derivative have been calculated using integration by parts. For linear propensity functions, the second term on the right-hand side can be rewritten into the required covariances. For simplicity, the focus lies on unimolecular reactions obeying mass action kinetics, i.e. propensity functions of the form $\lambda_k(\bar{z}(t),x(t)) = c_k z_{l(k)}(t)$, where $Z_{l(k)}$ denotes the species triggering reaction $k$. Equivalent statements hold for linearised propensity functions depending on more than one species as well. With this kind of propensity functions, Eq. (G.2) can be written as

$$\mathrm{d}\langle\bar{z}_i(t)\mid x_0^t\rangle = \sum_{k\in R_{\bar{z}_i}} s_{\bar{z}_i,k}c_k\langle z_{l(k)}(t)\mid x_0^t\rangle\mathrm{d}t + \sum_{k\in R_x}\frac{c_k\mathrm{Cov}\left[\bar{z}_i(t),z_{l(k)}(t)\mid x_0^t\right]}{\sigma_k}\mathrm{d}w_k(t) + \sum_{k\in R_{\bar{z}_i}\cap R_{\bar{x}}} s_{\bar{z}_i,k}\sigma_k\mathrm{d}w_k(t), \tag{G.3}$$

where we used that the conditional covariance is non-zero only for reactions in $R_x$. The latter can now be used to formulate an equation for the differential of the product $\langle \bar{z}_i(t) \mid x_0^t \rangle \langle \bar{z}_j(t) \mid x_0^t \rangle$. From Ito's lemma, it follows

$$
\begin{aligned}
\mathrm{d}\left(\langle \bar{z}_i(t) \mid x_0^t \rangle \langle \bar{z}_j(t) \mid x_0^t \rangle\right) = & \sum_{k \in R_{\bar{z}_i}} s_{\bar{z}_i,k} c_k \langle \bar{z}_j(t) \mid x_0^t \rangle \langle z_{l(k)}(t) \mid x_0^t \rangle \mathrm{d}t + \sum_{k \in R_{\bar{z}_j}} s_{\bar{z}_j,k} c_k \langle \bar{z}_i(t) \mid x_0^t \rangle \langle z_{l(k)}(t) \mid x_0^t \rangle \mathrm{d}t \\
& + \sum_{k \in R_x \setminus (R_{\bar{z}_i} \cup R_{\bar{z}_j})} c_k^2 \frac{\mathrm{Cov}[\bar{z}_i(t), z_{l(k)}(t) \mid x_0^t] \mathrm{Cov}[\bar{z}_j(t), z_{l(k)}(t) \mid x_0^t]}{\sigma_k^2} \mathrm{d}t \\
& + \sum_{k \in (R_{\bar{z}_i} \cup R_{\bar{z}_j}) \cap R_{\tilde{x}}} \left( \frac{c_k \mathrm{Cov}[\bar{z}_i(t), z_{l(k)}(t) \mid x_0^t]}{\sigma_k} + s_{\bar{z}_i,k} \sigma_k \right) \cdot \left( \frac{c_k \mathrm{Cov}[\bar{z}_j(t), z_{l(k)}(t) \mid x_0^t]}{\sigma_k} + s_{\bar{z}_j,k} \sigma_k \right) \mathrm{d}t \\
& + \sum_{k \in R_x \setminus R_{\bar{z}_i}} \langle \bar{z}_j(t) \mid x_0^t \rangle \frac{c_k \mathrm{Cov}[\bar{z}_i(t), z_{l(k)}(t) \mid x_0^t]}{\sigma_k} \mathrm{d}w_k(t) \\
& + \sum_{k \in R_{\bar{z}_i} \cap R_{\tilde{x}}} \langle \bar{z}_j(t) \mid x_0^t \rangle \left( \frac{c_k \mathrm{Cov}[\bar{z}_i(t), z_{l(k)}(t) \mid x_0^t]}{\sigma_k} + s_{\bar{z}_i,k} \sigma_k \right) \mathrm{d}w_k(t) \\
& + \sum_{k \in R_x \setminus R_{\bar{z}_j}} \langle \bar{z}_i(t) \mid x_0^t \rangle \frac{c_k \mathrm{Cov}[\bar{z}_j(t), z_{l(k)}(t) \mid x_0^t]}{\sigma_k} \mathrm{d}w_k(t) \\
& + \sum_{k \in R_{\bar{z}_j} \cap R_{\tilde{x}}} \langle \bar{z}_i(t) \mid x_0^t \rangle \left( \frac{c_k \mathrm{Cov}[\bar{z}_j(t), z_{l(k)}(t) \mid x_0^t]}{\sigma_k} + s_{\bar{z}_j,k} \sigma_k \right) \mathrm{d}w_k(t).
\end{aligned}
\tag{G.4}
$$

Analogously to Eq. (G.2), we can derive a differential equation for the second conditional moment as

$$
\begin{aligned}
\mathrm{d}\langle \bar{z}_i(t) \bar{z}_j(t) \mid x_0^t \rangle = & \sum_{k \in R_{\tilde{Z}_i}} s_{\bar{z}_i,k} c_k \langle \bar{z}_j(t) z_{l(k)}(t) \mid x_0^t \rangle \mathrm{d}t + \sum_{k \in R_{\tilde{Z}_j}} s_{\bar{z}_j,k} c_k \langle \bar{z}_i(t) z_{l(k)}(t) \mid x_0^t \rangle \mathrm{d}t \\
& + \sum_{k \in R_{\tilde{Z}_j} \cap R_{\tilde{Z}_i}} s_{\bar{z}_i,k} s_{\bar{z}_j,k} \sigma_k^2 \mathrm{d}t + \sum_{k \in R_{\tilde{X}}} \frac{c_k \langle \bar{z}_i(t) \bar{z}_j(t) z_{l(k)}(t) \mid x_0^t \rangle - c_k \langle \bar{z}_i(t) \bar{z}_j(t) \mid x_0^t \rangle \langle z_{l(k)}(t) \mid x_0^t \rangle}{\sigma_k} \mathrm{d}w_k(t) \\
& + \sum_{k \in R_{\tilde{Z}_i} \cap R_{\tilde{X}}} s_{\bar{z}_i,k} \sigma_k \langle \bar{z}_j(t) \mid x_0^t \rangle \mathrm{d}w_k(t) + \sum_{k \in R_{\tilde{Z}_j} \cap R_{\tilde{X}}} s_{\bar{z}_j,k} \sigma_k \langle \bar{z}_i(t) \mid x_0^t \rangle \mathrm{d}w_k(t).
\end{aligned}
\tag{G.5}
$$

Subtracting Eq. (G.4) from Eq. (G.5), and using that the third central moment of the Gaussian distribution vanishes, which implies

$$
\begin{aligned}
\langle \bar{z}_i(t) \bar{z}_j(t) \bar{z}_m(t) \mid x_0^t \rangle = & \langle \bar{z}_i(t) \mid x_0^t \rangle \langle \bar{z}_j(t) \bar{z}_m(t) \mid x_0^t \rangle + \langle \bar{z}_j(t) \mid x_0^t \rangle \langle \bar{z}_i(t) \bar{z}_m(t) \mid x_0^t \rangle \\
& + \langle \bar{z}_m(t) \mid x_0^t \rangle \langle \bar{z}_i(t) \bar{z}_j(t) \mid x_0^t \rangle - 2 \langle \bar{z}_i(t) \mid x_0^t \rangle \langle \bar{z}_j(t) \mid x_0^t \rangle \langle \bar{z}_m(t) \mid x_0^t \rangle,
\end{aligned}
\tag{G.6}
$$

we obtain an expression for the conditional covariance as

$$
\begin{aligned}
\mathrm{d}\mathrm{Cov}[\bar{z}_i(t), \bar{z}_j(t) \mid x_0^t] = & \mathrm{d}\langle \bar{z}_i(t) \bar{z}_j(t) \mid x_0^t \rangle - \mathrm{d}\left(\langle \bar{z}_i(t) \mid x_0^t \rangle \langle \bar{z}_j(t) \mid x_0^t \rangle\right) \\
= & \sum_{k \in R_{\bar{z}_i}} s_{\bar{z}_i,k} c_k \mathrm{Cov}[\bar{z}_j(t), z_{l(k)}(t) \mid x_0^t] \mathrm{d}t + \sum_{k \in R_{\bar{z}_j}} s_{\bar{z}_j,k} c_k \mathrm{Cov}[\bar{z}_i(t), z_{l(k)}(t) \mid x_0^t] \mathrm{d}t \\
& + \sum_{k \in R_{\bar{z}_i} \cap R_{\bar{z}_j}} s_{\bar{z}_i,k} s_{\bar{z}_j,k} \sigma_k^2 \mathrm{d}t \\
& - \sum_{k \in R_{\tilde{x}}} \left( \frac{c_k \mathrm{Cov}[\bar{z}_i(t), z_{l(k)}(t) \mid x_0^t]}{\sigma_k} + s_{\bar{z}_i,k} \sigma_k \right) \cdot \left( \frac{c_k \mathrm{Cov}[\bar{z}_j(t), z_{l(k)}(t) \mid x_0^t]}{\sigma_k} + s_{\bar{z}_j,k} \sigma_k \right) \mathrm{d}t.
\end{aligned}
\tag{G.7}
$$

Interestingly, (G.7) depends neither on Wiener increments nor the conditional mean. This means that the conditional covariance evolves deterministically, which is the case also in the conventional Kalman-Bucy filter [14]. Hence, it follows

$$
\left\langle \mathrm{Cov}[\bar{z}_i(t), z_{l(k)}(t) \mid x_0^t] \mathrm{Cov}[\bar{z}_j(t), z_{l(k)}(t) \mid x_0^t] \right\rangle = \left\langle \mathrm{Cov}[\bar{z}_i(t), z_{l(k)}(t) \mid x_0^t] \right\rangle \left\langle \mathrm{Cov}[\bar{z}_j(t), z_{l(k)}(t) \mid x_0^t] \right\rangle. \tag{G.8}
$$

We therefore obtain for the expected conditional covariance

$$
\begin{aligned}
\mathrm{d}\big\langle \mathrm{Cov}[\bar z_i(t),\bar z_j(t)\mid x_0^t]\big\rangle =& \mathrm{d}\langle \bar z_i(t)\bar z_j(t)\rangle - \mathrm{d}\big\langle\langle \bar z_i(t)\mid x_0^t\rangle\langle \bar z_j(t)\mid x_0^t\rangle\big\rangle \\
=& \sum_{k\in R_{\bar z_i}} s_{\bar z_i,k}c_k\big\langle \mathrm{Cov}[\bar z_j(t), z_{l(k)}(t)\mid x_0^t]\big\rangle \mathrm{d}t + \sum_{k\in R_{\bar z_j}} s_{\bar z_j,k}c_k\big\langle \mathrm{Cov}[\bar z_i(t), z_{l(k)}(t)\mid x_0^t]\big\rangle \mathrm{d}t \\
&+ \sum_{k\in R_{\bar z_i}\cap R_{\bar z_j}} s_{\bar z_i,k}s_{\bar z_j,k}\sigma_k^2 \mathrm{d}t \\
&- \sum_{k\in R_{\bar x}} \Big(\frac{c_k\big\langle \mathrm{Cov}[\bar z_i(t), z_{l(k)}(t)\mid x_0^t]\big\rangle}{\sigma_k} + s_{\bar z_i,k}\sigma_k\Big)\cdot\Big(\frac{c_k\big\langle \mathrm{Cov}[\bar z_j(t), z_{l(k)}(t)\mid x_0^t]\big\rangle}{\sigma_k} + s_{\bar z_j,k}\sigma_k\Big)\mathrm{d}t.
\end{aligned}
\tag{G.9}
$$

Note that if $z_{l(k)}(t)\in x(t)$, the corresponding conditional covariance is zero. The dependence of one covariance on other covariances results in a system of differential equations the size of which scales with the number of hidden species. To simplify the form of Eq. (G.9), the latter can be written in matrix form, which at the same time, yields a method to evaluate all required covariances of the system. Defining the matrix element $K_{ij} = \langle \mathrm{Cov}[\bar z_i(t),\bar z_j(t)\mid x_0^t]\rangle$, the final result reads

$$
\mathrm{d}K = SCR^T K\mathrm{d}t + KRCS^T\mathrm{d}t + S\Sigma^2S^T\mathrm{d}t - \big(KR\bar\Sigma^x C + S\Sigma^x\big)\cdot\Big(C\bar\Sigma^x R^T K + \Sigma^x S^T\Big)\mathrm{d}t,
\tag{G.10}
$$

which corresponds to Eq. (6) of the main text. Here, $S$ is the net stoichiometry matrix of species $\bar{\mathrm{Z}}$ with dimension $M_{\bar Z}\times K$, $M_{\bar Z}$ the number of species $\bar{\mathrm{Z}}$ and $R$ is the reactant stoichiometry matrix with same dimensions as $S$. The matrix $C$ is a diagonal matrix with the rate constants as its diagonal elements, i.e. $C_{k,k}=c_k$, $\Sigma$ is a diagonal matrix with entries $\Sigma_{k,k}=\sigma_k$ and the matrices $\Sigma^x$ and $\bar\Sigma^x$ are variants of $\Sigma$ with entries $\Sigma^x_{k,k}=\sigma_k$ and $\bar\Sigma^x k,k = 1/\sigma_k$, respectively, if $k\in R_{\bar x}$ and 0 otherwise. Solving Eq. (G.10) provides expressions for the expected conditional variances, which allows us to calculate the reaction-based path mutual information in Eq. (D.9).

## H. On the magnitude of the Path Mutual Information

In this section, we want to show that the reaction-based path mutual information rate is larger or equal to the state-based path mutual information rate, provided that the latter is well-defined. The key is to understand how the noise strengths enter the filtering equation and the path mutual information in the respective regimes. Recall that the filtering equation in the reaction-based description (Eq. (5) main text) is given by

$$
\mathrm{d}\pi^x(\bar z,t) = \mathscr{A}\pi^x(\bar z,t)\mathrm{d}t + \pi^x(\bar z,t)\sum_{k\in R_{\bar x}}\frac{\lambda_k(\bar z,x(t)) - \langle\lambda_k(\bar z(t),x(t))\mid x_0^t\rangle}{\sigma_k}\mathrm{d}w_k(t) - \sum_{k\in R_{\bar z}\cap R_{\bar x}} s^T_{\bar z,k}\sigma_k\partial_{\bar z}\tilde\pi^x(\bar z,t)\mathrm{d}w_k(t)
\tag{H.1}
$$

The filtering equation in the state-based description can be written as

$$
\mathrm{d}\pi^{\tilde x} = \mathscr{A}\pi^{\tilde x}\mathrm{d}t + \frac{\sum_{k\in R_{\bar x}}\big(\lambda_k(\bar z,x(t)) - \langle\lambda_k(\bar z(t),x(t))\mid \tilde x_0^t\rangle\big)}{\sigma_x}\pi^{\tilde x}\mathrm{d}w(t)
\tag{H.2}
$$

where $\tilde x_0^t$ defines the state-based path of $x(t)$ and $\sigma_x = \sqrt{\sum_{k\in R_{\bar x}} s^2_{x,k}h_k(\hat z^*)}$ [17]. The state-based path mutual information can be ill-defined in cases where $\bar z(t)$ and $x(t)$ change simultaneously. Therefore, we focus on systems where $R_{\bar x}\cap R_{\bar z}=\emptyset$. For our purposes, we restrict ourselves to the two-species case, i.e. $\bar z(t) = y(t)$, and systems where we have only one reaction in $R_x$ with propensity $\lambda_l(\bar z(t),x(t)) = c_l\bar z(t)$ and $R_y=\emptyset$, for instance $\bar{\mathrm{Z}}\to\mathrm{X}$. Under these conditions, the mutual information rate between the reaction-based paths $x_0^t$ and $\bar z_0^t$, the integrand of Eq. (4), main text, simplifies to

$$
i_t^{x\bar z} = \frac{1}{2}\frac{c_l^2\langle \mathrm{Var}[\bar z(s)\mid x_0^t]\rangle}{\sigma_l^2}
\tag{H.3}
$$

as $\langle \mathrm{Var}[\bar z(s)\mid x_0^t,\bar z_0^t]\rangle = 0$. Analogously, the mutual information rate between the state-based paths $\tilde x_0^t$ and $\tilde z_0^t$, the integrand of Eq. (3), becomes

$$
i_t^{\tilde x\tilde z} = \frac{1}{2}\frac{c_l^2\langle \mathrm{Var}[\bar z(s)\mid \tilde x_0^t]\rangle}{\sigma_x^2}.
\tag{H.4}
$$

The key is to show that $c_l^2\langle \mathrm{Var}[\bar z(s)\mid x_0^t]\rangle/\sigma_l^2 \geq c_l^2\langle \mathrm{Var}[\bar z(s)\mid \tilde x_0^t]\rangle/\sigma_x^2$. Following the derivation steps in SM G, we obtain for the expected conditional variance in the reaction-based description

$$
\mathrm{d}\big\langle \mathrm{Var}[\bar z(t)\mid x_0^t]\big\rangle = \sum_{k\in R_{\bar z}} s_{\bar z,k}c_k\big\langle \mathrm{Var}[\bar z(t)\mid x_0^t]\big\rangle\mathrm{d}t + \sum_{k\in R_{\bar z}} s^2_{\bar z,k}\sigma_k^2\mathrm{d}t - \Big(\frac{c_l\big\langle \mathrm{Var}[\bar z(t)\mid x_0^t]\big\rangle}{\sigma_l}\Big)^2\mathrm{d}t.
\tag{H.5}
$$

Equivalently, the state-based expected conditional covariance reads [17]

$$\mathrm{d}\left\langle \mathrm{Var}[\bar{z}(t) \mid \vec{x}_0^t]\right\rangle = \sum_{k\in R_{\bar{z}}} s_{\bar{z},k}c_k \left\langle \mathrm{Var}[\bar{z}(t) \mid \vec{x}_0^t]\right\rangle \mathrm{d}t + \sigma_{\bar{z}}^2 \mathrm{d}t - \left(\frac{c_l \left\langle \mathrm{Var}[\bar{z}(t) \mid \vec{x}_0^t]\right\rangle}{\sigma_x}\right)^2 \mathrm{d}t. \tag{H.6}$$

Here, $\sigma_{\bar{z}}^2 := \sum_{k\in R_{\bar{z}}} s_{\bar{z},k}^2 \sigma_k^2$ denotes the noise strength of $\bar{z}(t)$. Solving Eq. (H.5) and Eq. (H.6) in steady state, yields

$$\left\langle \mathrm{Var}[\bar{z}(t) \mid x_0^t]\right\rangle = \frac{\sigma_l^2}{c_l^2}\left(\frac{1}{2}\sum_{k\in R_{\bar{z}}} s_{\bar{z},k}c_k \pm \sqrt{\left(\frac{1}{2}\sum_{k\in R_{\bar{z}}} s_{\bar{z},k}c_k\right)^2 + c_l^2 \frac{\sigma_{\bar{z}}^2}{\sigma_l^2}}\right) \tag{H.7}$$

for the reaction-based case and

$$\left\langle \mathrm{Var}[\bar{z}(t) \mid \vec{x}_0^t]\right\rangle = \frac{\sigma_x^2}{c_l^2}\left(\frac{1}{2}\sum_{k\in R_{\bar{z}}} s_{\bar{z},k}c_k \pm \sqrt{\left(\frac{1}{2}\sum_{k\in R_{\bar{z}}} s_{\bar{z},k}c_k\right)^2 + c_l^2 \frac{\sigma_{\bar{z}}^2}{\sigma_x^2}}\right) \tag{H.8}$$

for the state-based case. Inserting these results into the expressions for the mutual information rate, we obtain for the reaction-based case

$$i_{\mathrm{rb}}^{x\bar{z}} = \frac{1}{2}\sum_{k\in R_{\bar{z}}} s_{\bar{z},k}c_k \pm \sqrt{\left(\frac{1}{2}\sum_{k\in R_{\bar{z}}} s_{\bar{z},k}c_k\right)^2 + c_l^2 \frac{\sigma_{\bar{z}}^2}{\sigma_l^2}} \tag{H.9}$$

and for the state-based one

$$i_{\mathrm{sb}}^{x\bar{z}} = \frac{1}{2}\sum_{k\in R_{\bar{z}}} s_{\bar{z},k}c_k \pm \sqrt{\left(\frac{1}{2}\sum_{k\in R_{\bar{z}}} s_{\bar{z},k}c_k\right)^2 + c_l^2 \underbrace{\frac{\sigma_{\bar{z}}^2}{\sigma_x^2}}_{\leq \sigma_{\bar{z}}^2/\sigma_l^2}}. \tag{H.10}$$

Hence, $i_{\mathrm{rb}}^{x\bar{z}} \geq i_{\mathrm{sb}}^{x\bar{z}}$. Importantly, the inequality becomes a true inequality if $R_x \subseteq R_{\bar{x}}$ is a proper subset.

## I. Motif a

In this section, we want to show explicitly how the state-based and reaction-based descriptions of a path lead to different results for the mutual information rate of Motif a in Table 1. Recall that Motif a follows the network structure

$$\emptyset \xrightarrow{c_1} \mathrm{A} \qquad \mathrm{A} \xrightarrow{c_2 A(t)} \emptyset$$
$$\mathrm{A} \xrightarrow{c_3 A(t)} \mathrm{A}+\mathrm{B} \qquad \mathrm{B} \xrightarrow{c_4 B(t)} \emptyset. \tag{I.1}$$

For $a(t)$ and $b(t)$ being Gaussian processes, we can write the time-evolution of them according to Eq. (A.6) and Eq. (A.5) as

$$\begin{aligned}
\mathrm{d}(\delta a(t)) &= c_1 - c_2\delta a(t) + \sqrt{c_1}\mathrm{d}w_1(t) - \sqrt{c_2 a^*}\mathrm{d}w_2(t)\\
&= c_1 - c_2\delta a(t) + \sqrt{c_1 + c_2 a^*}\mathrm{d}w_a(t)\\
\mathrm{d}(\delta b(t)) &= c_3\delta a(t) - c_4\delta b(t) + \underbrace{\sqrt{c_3 a^*}}_{\sigma_3}\mathrm{d}w_3(t) - \underbrace{\sqrt{c_4 b^*}}_{\sigma_4}\mathrm{d}w_4(t)\\
&= c_3\delta a(t) - c_4\delta b(t) + \underbrace{\sqrt{c_3 a^* + c_4 b^*}}_{\sigma_b}\mathrm{d}w_b(t),
\end{aligned} \tag{I.2}$$

where the first line of the dynamics of $b(t)$ corresponds to a reaction-based description and the second to a state-based. Considering that $b^* = c_3 a^*/c_4$, we obtain $\sigma_b = \sqrt{2c_3 a^*} = \sqrt{2}\sigma_3$. The path mutual information rate between $a_0^t$ and $b_0^t$ is given by

$$i_t^{ab} = \frac{c_3^2}{2}\frac{\langle \mathrm{Var}[a(t) \mid b_0^t]\rangle}{\sigma^2}, \tag{I.3}$$

where $\sigma = \sigma_3$ in the case of a reaction-based description and $\sigma = \sigma_b$ in case of a state-based description. In order to solve Eq. (I.3), we need an expression for the expected conditional variance. In the state-based description, this can be derived with a Kalman Filter [15]. For the reaction-based case, we use Eq. (6), main text, to derive an expression for the time-evolution of $\langle \mathrm{Var}[a(t) \mid b_0^t]\rangle$. Here, we look at the conditional system given the path of $b(t)$. Then, the required matrices for this system are given by

$$S = \begin{pmatrix}1 & -1 & 0 & 0\end{pmatrix} \tag{I.4}$$

$$R = \begin{pmatrix}0 & 1 & 1 & 0\end{pmatrix} \tag{I.5}$$

$$C = \begin{pmatrix} c_1 & 0 & 0 & 0 \\ 0 & c_2 & 0 & 0 \\ 0 & 0 & c_3 & 0 \\ 0 & 0 & 0 & c_4 \end{pmatrix} \tag{I.6}$$

$$\Sigma = \begin{pmatrix} \sigma_1 & 0 & 0 & 0 \\ 0 & \sigma_2 & 0 & 0 \\ 0 & 0 & \sigma_3 & 0 \\ 0 & 0 & 0 & \sigma_4 \end{pmatrix} \tag{I.7}$$

$$\Sigma^b = \begin{pmatrix} 0 & 0 & 0 & 0 \\ 0 & 0 & 0 & 0 \\ 0 & 0 & \sigma_3 & 0 \\ 0 & 0 & 0 & \sigma_4 \end{pmatrix} \tag{I.8}$$

$$\sigma^b = \begin{pmatrix} 0 & 0 & 0 & 0 \\ 0 & 0 & 0 & 0 \\ 0 & 0 & 1/\sigma_3 & 0 \\ 0 & 0 & 0 & 1/\sigma_4 \end{pmatrix} \tag{I.9}$$

Due to the linearity of motif a and the fact that species A and B do not change simultaneously, the resulting expected conditional variances in each description follow the same structure, and only differ in the noise strength $\sigma$. From the Kalman filter [14], we obtain

$$\begin{aligned} \frac{\mathrm{d}}{\mathrm{d}t}\langle \mathrm{Var}[a(t) \mid b_0^t]\rangle =& c_1 + c_2 a^* - 2c_2 \langle \mathrm{Var}[a(t) \mid b_0^t]\rangle \\ & - \frac{c_3^2 \langle \mathrm{Var}[a(t) \mid b_0^t]\rangle^2}{\sigma^2}. \end{aligned} \tag{I.10}$$

Now, we can combine Eq. (I.3) and Eq. (I.10) in steady state to obtain an expression for the stationary path mutual information rate dependent on $\sigma$. Considering $a^* = c_1/c_2$ yields

$$i^{ab}(\sigma) = -\frac{c_2}{2} + \frac{1}{2}\sqrt{c_2^2 + \frac{2c_1c_3^2}{\sigma^2}}. \tag{I.11}$$

With a state-based path description, we insert $\sigma = \sigma_b$ and the factor of 2 cancels. With a reaction-based path description, instead, we insert $\sigma = \sigma_3$ and the factor of 2 remains.

## J. Mutual Information in the Receptor-Ligand Binding System

For Case Study II, we calculated the stationary path mutual information rate between a ligand L and the two receptor states $R_b$ and $R_u$ which are connected via the network

$$\begin{aligned} &\emptyset \xrightarrow{c_1} \mathrm{L} && \mathrm{L} \xrightarrow{c_2 l(t)} \emptyset \\ &\mathrm{L} + \mathrm{R_u} \xrightarrow{c_+ l(t) r_\mathrm{u}(t)} \mathrm{L} + \mathrm{R_b} && \mathrm{R_b} \xrightarrow{c_- r_\mathrm{b}(t)} \mathrm{R_u}, \end{aligned} \tag{J.1}$$

where $c_1, c_2, c_-, c_+ \in \mathbb{R}_{\geq 0}$. The copy numbers of the respective components are given by $l(t)$, $r_\mathrm{b}(t)$ and $r_\mathrm{u}(t)$. The total copy number of receptors is given by the sum $r_T = r_\mathrm{b}(t) + r_\mathrm{u}(t)$ and is constant. We calculated the mutual information rate once in the reaction-based and once in the state-based description. In the following, we present the detailed calculations to obtain the results shown in the main text.

### J.1. Reaction-Based Mutual Information

The mutual information rate between the reaction-based paths of the ligand and the ligand-bound receptor is given by

$$i_\mathrm{rb}^{lr} = \frac{1}{2}\frac{c_+(r_T - r_b^*)\left\langle \mathrm{Var}[l(t) \mid (r_\mathrm{b})_0^t]\right\rangle}{l^*}. \tag{J.2}$$

For calculating the stationary rate, we therefore need to calculate the stationary conditional variance of $l(t)$ given $(r_\mathrm{b})_0^t$. According to Eq. (6), main text, we can write

$$\frac{\mathrm{d}}{\mathrm{d}t}\langle \mathrm{Var}[l(t) \mid (r_\mathrm{b})_0^t]\rangle = c_1 + c_2 l^* - 2c_2 \langle \mathrm{Var}[l(t) \mid (r_\mathrm{b})_0^t]\rangle - \frac{c_+(r_T - r_\mathrm{b}^*)\langle \mathrm{Var}[l(t) \mid (r_\mathrm{b})_0^t]\rangle^2}{l^*}. \tag{J.3}$$

Solving this in steady state yields

$$\langle \mathrm{Var}[l(t) \mid (r_\mathrm{b})_0^t]\rangle^* = -\frac{c_1(c_1c_+ + c_2c_-)}{c_2c_+c_-r_T} + \frac{c_1\sqrt{(c_1c_+ + c_2c_-)(c_1c_+ + c_2c_- + 2c_-c_+r_T)}}{c_2c_+c_-r_T} \tag{J.4}$$

Inserting the latter in the expression for the mutual information rate and considering $l^* = c_1/c_2$ and $r_a^* = r_T c_+ l^*/(c_+ l^* + c_-)$, we obtain

$$i_{\rm rb}^{lr} = -\frac{c_2}{2} + \frac{c_2}{2}\sqrt{\frac{2r_T c_- c_+}{c_2 c_- + c_1 c_+} + 1}. \tag{J.5}$$

Defining $T = 1/c_2$, $\bar{n}_b = Tp/\bar{\tau}_b$, $\bar{\tau}_b = 1/c_-$ and $p = r_b^*/r_T$ as stated in the main text leads to Eq. (9) of the main text.

## J.2. State-Based Mutual Information

For calculating the mutual information rate between state-based paths in this system, we write the Chemical Langevin Equation under the Linear-Noise Approximation according to (Eq. (A.6)) as

$$\mathrm{d}l(t) = c_1 \mathrm{d}t - c_2 l(t)\mathrm{d}t + \underbrace{\sqrt{c_1 + c_2 l^*}}_{2c_1}\mathrm{d}w(t) \tag{J.6}$$

for the ligand, where $l^* = c_1/c_2$ defines the steady state copy number of the macroscopic mean of $l(t)$, and for the receptor in the on-state

$$\begin{aligned}\mathrm{d}r_{\rm b}(t) =& c_+ \left(r_T - r_{\rm b}^*\right) l(t)\mathrm{d}t + c_+ l^* \left(r_T - r_{\rm b}(t)\right)\mathrm{d}t - c_- r_{\rm b}(t)\mathrm{d}t \\ &+ \sqrt{c_+\left(r_T - r_{\rm b}^*\right) l^* + c_- r_{\rm a}^*}\mathrm{d}w(t)\end{aligned} \tag{J.7}$$

where $r_{\rm b}^* = r_T c_+ l^*/(c_+ l^* + c_-)$ denotes the steady state copy number of the macroscopic mean of $r_{\rm b}(t)$. Defining the rate constants

$$\begin{aligned}\rho &= c_+ r_T \frac{c_-}{c_+ l^* + c_-} \\ \mu &= c_+ l^* + c_-\end{aligned} \tag{J.8}$$

we can rewrite the dynamics of $r_{\rm b}(t)$ as z

$$\mathrm{d}r_{\rm b}(t) = \rho l(t)\mathrm{d}t - \mu r_{\rm b}(t)\mathrm{d}t + \underbrace{\sqrt{2\rho l^*}}_{\sqrt{2r_T p(1-p)\mu}}\mathrm{d}w(t). \tag{J.9}$$

Note that $p = r_{\rm b}^*/r_T = c_+ l^*/(c_+ l^* + c_-)$. This result for the noise strength in a ligand-receptor binding system has also been obtained in [18]. We observe that the linearised system can be redefined in a way that results in a structure analogous to the one of motif a, i.e. $\rho \sim c_3$. As the total copy number of receptors is conserved, in the linearised form the effective decay rate $\mu$ depends on both unbinding and binding. Therefore, we can easily see that the mutual information rate is given by

$$i_{\rm sb}^{lr} = -\frac{c_2}{2} + \frac{1}{2}\sqrt{c_2(c_2 + \rho)}. \tag{J.10}$$

Inserting the definition of $\rho$ and minor algebraic manipulations yield

$$i_{\rm sb}^{lr} = -\frac{c_2}{2} + \frac{c_2}{2}\sqrt{\frac{r_T c_- c_+}{c_2 c_- + c_1 c_+} + 1}. \tag{J.11}$$

Again, defining $T = 1/c_2$, $\bar{n}_b = Tp/\bar{\tau}_b$, $\bar{\tau}_b = 1/c_-$ and $p = r_{\rm b}^*/r_T$ leads to Eq. (10) of the main text.

## J.3. Interpretation of the Mutual Information Rate

Based on the definitions in Eq. (J.8), we can rewrite the mutual information rate in both formalisms given by Eq. (J.5) and Eq. (J.11) in a form that allows an intuitive interpretation, similar to the one in the main text (Eqs. (9-10)). Noting that the correlation time of the input signal $l(t)$ is given by $\tau_l \equiv 1/c_2$, we can rewrite Eqs. (J.8) and (J.5) as

$$\begin{aligned}i_{\rm rb}^{lr} &= \frac{1}{2\tau_l}\left(\sqrt{2\rho\tau_l + 1} - 1\right) \\ i_{\rm sb}^{lr} &= \frac{1}{2\tau_l}\left(\sqrt{\rho\tau_l + 1} - 1\right)\end{aligned} \tag{J.12}$$

Exploiting that $\rho = (1-p)r_T c_+$ and the receptor occupancy $p = c_+ l^*/\mu$ with $\mu = c_- + c_+ l^*$, these equations can be rewritten as

$$\begin{aligned}i_{\rm rb}^{lr} &= \frac{1}{2\tau_l}\left(\sqrt{2r_T p(1-p)\mu\frac{\tau_l}{l^*} + 1} - 1\right) \\ i_{\rm sb}^{lr} &= \frac{1}{2\tau_l}\left(\sqrt{r_T p(1-p)\mu\frac{\tau_l}{l^*} + 1} - 1\right)\end{aligned} \tag{J.13}$$

Interestingly, the relative *instantaneous* sensing error $\delta l_{\rm ins}/l^*$ based on $r_T$ independent measurements by $r_T$ receptors is given by

$$\left(\frac{\delta l_{\rm ins}}{l^*}\right)^2 = \frac{1}{p(1-p)r_T}, \tag{J.14}$$

which is a classical result in the field of chemical sensing [19]. Moreover, $\mu$ is given by the inverse of the correlation time, i.e. $\mu = 1/\tau_c$. For our signal, we find $\mathrm{Var}[l(t)] = l^*$. Inserting these expressions into Eq. (J.13) yields

$$\begin{aligned} i^{lr}_{\rm rb} &= \frac{1}{2\tau_l}\left(\sqrt{2\frac{\mathrm{Var}[l(t)]}{\delta l^2_{\rm ins}}\frac{\tau_l}{\tau_c}+1}-1\right) \\ i^{lr}_{\rm sb} &= \frac{1}{2\tau_l}\left(\sqrt{\frac{\mathrm{Var}[l(t)]}{\delta l^2_{\rm ins}}\frac{\tau_l}{\tau_c}+1}-1\right). \end{aligned} \tag{J.15}$$

Here, $\delta l^2_{\rm ins}/(\tau_l/\tau_c)$ is the Berg-Purcell sensing error squared based on integrating the receptor state over the timescale of the input correlation time $\tau_l$. It is given by the instantaneous error squared $\delta l^2_{\rm ins}$ divided by the number of independent concentration measurements on the input timescale $\tau_l$, given by $\tau_l/\tau_c$ [19]. The squared sensing error with Maximum-Likelihood sensing is smaller by a factor of 2 as compared to Berg-Purcell sensing [20], explaining the factor-of-two difference in the expressions for the rate between the state-based and reaction-based description of the input and output trajectories. Eq. (J.15) shows that the information rate is given by the time scale $\tau_l$ on which new independent concentration levels are transmitted times the number of concentration levels that can be resolved, which is determined by the standard deviation of the input over the error, which is $\sqrt{\mathrm{Var}[l(t)]}/(\delta l_{\rm ins}/\sqrt{\tau_l/\tau_c})$ for the state-based and $\sqrt{\mathrm{Var}[l(t)]}/(\delta l_{\rm ins}/\sqrt{2\tau_l/\tau_c})$ for the reaction-based formalism. Finally, we note that the error $\delta l_{\rm ins}$ defined here is the instantaneous error based on $r_T$ independent measurements, while the error $\delta l$ defined in the main text is that of a single receptor read out over an integration time $\tau_l$.

### J.4. Multi-State Receptor

In the main text, we calculate the mutual information rate between the ligand and a multi-state receptor $i^{lr}_{\rm ms}$ between state-based paths. As this can become analytically challenging for a large number of receptor states, we obtain $i^{lr}_{\rm ms}$ by calculating the reaction-based mutual information rate $i^{lx}$ between the ligand and a fast downstream species X. In the limit of very fast production and degradation of X, this is equivalent to the state-based mutual information rate $i^{lr}_{\rm ms}$. We calculate $i^{lr}_{\rm ms}$ numerically using an automated Python script. The network including the multi-state receptor is given by

$$\begin{aligned} &\emptyset \xrightarrow{c_1} \mathrm{L} && \mathrm{L}+\mathrm{R_u} \xrightarrow{c_+ l(t) r_{\rm u}(t)} \mathrm{L}+\mathrm{R_{b,1}} \\ &\mathrm{L} \xrightarrow{c_2 l(t)} \emptyset && \mathrm{R_{b,1}} \xrightarrow{\mu r_{\rm b,1}(t)} \mathrm{R_{b,2}} \xrightarrow{\mu r_{\rm b,2}(t)} \dots \xrightarrow{\mu r_{{\rm b},N-1}(t)} \mathrm{R}_{{\rm b},N} \\ &\mathrm{R}_{{\rm b},N} \xrightarrow{c_- r_{{\rm b},N}(t)} \mathrm{R_u} && \mathrm{R}_{{\rm b},i} \xrightarrow{c_4 r_{{\rm b},i}(t)} \mathrm{X} \\ &\mathrm{X} \xrightarrow{c_5 x(t)} \emptyset. \end{aligned} \tag{J.16}$$

The mutual information rate between the paths $l_0^t$ and $x_0^t$ in the reaction-based description is given by

$$i^{lx}_t = \sum_{i=1}^{N} \frac{c_4}{2} \frac{\langle \mathrm{Var}[r_{{\rm b},i}(t) \mid x_0^t]\rangle - \langle \mathrm{Var}[r_{{\rm b},i}(t) \mid x_0^t, l_0^t]\rangle}{r^*_{{\rm b},i}}, \tag{J.17}$$

where $r^*_{{\rm b},i}$ denotes the steady state value of the macroscopic means of the active receptor states. For obtaining the state-based mutual information rate $i^{lr}_{\rm ms}$ from $i^{lx}_t$, we define a reaction velocity $v_X$ as $c_4 = v_X\tilde{k}_4$ and $c_5 = v_X\tilde{k}_5$, where $\tilde{k}_4$ and $\tilde{k}_5$ are non-negative constants. In the limit of $v_X \to \infty$ and in steady state, we obtain $\lim_{t\to\infty} i^{lx}_t \xrightarrow{v_X\to\infty} i^{lr}_{\rm ms}$. For this calculation, we set $\{c_4, c_5\} = \{500, 50\}$ as in this regime we already observed convergence. For the remaining calculations we refer to the provided Python script.

## K. General Multi-State Signalling Motif

To underline the generality of our results in Case Study II of the main text, we here present the state-based path mutual information rate of a generic linear network motif comprising multiple readout states. This multi-state motif is based on the canonical motif a of the main text (Table 1), which is a linear representation of any signal A eliciting cellular response B. Instead of a single readout state B, the multi-state motif allows any number of intermediate states $\mathrm{B}_1$ to $\mathrm{B}_N$,

$$\begin{aligned} &A \xrightarrow{c_3} A + B_1, \\ &B_1 \xrightarrow{\mu} B_2 \xrightarrow{\mu} \dots \xrightarrow{\mu} B_N \xrightarrow{\mu} \emptyset, \end{aligned} \tag{K.1}$$

where for simplicity we have chosen the decay rate $\mu$ of each readout species to be equal. As in the main text, the signal A is generated by a birth death process:

$$\emptyset \underset{c_2}{\overset{c_1}{\rightleftharpoons}} A. \tag{K.2}$$

We consider the output of the network to be the sum of all readout states $b_T(t) = \sum_{i=1}^{N} b_i(t)$.

We can compute the state-based path mutual information rate between the input $a(t)$ and the output $b_T(t)$ via their corresponding (cross-)power spectra as shown in [12, 21],

$$i_{\text{sb}}^{ab_T} = -\frac{1}{4\pi}\int_{-\infty}^{\infty} d\omega \log\left(1 - \frac{|S_{ab_T}(\omega)|^2}{S_a(\omega)S_{b_T}(\omega)}\right). \tag{K.3}$$

Here, $S_x(\omega) = \lim_{t\to\infty} \frac{1}{t}|\tilde{x}_0^t(\omega)|^2$ denotes the power spectrum of a stationary species $X$, with $\tilde{x}(\omega)$ the Fourier transform of its abundance $x(t)$.

To obtain the required power spectra we exploit the Langevin form of the network dynamics. Using Eq. (A.6) we obtain for the signal A as defined in (K.1)

$$\dot{\delta a} = c_1 - c_2 a(t) + \sqrt{2c_2 a^*}\xi(t), \tag{K.4}$$

where $\xi(t)$ is a delta-correlated unit white noise process. The noise strength $\sqrt{2c_2a^*}$ follows from the reaction propensities as shown in Eq. (A.6) and exploiting that in steady state $c_1 = c_2 a^*$, with the mean signal concentration $a^*$. The power spectrum of the signal can now be obtained by taking the Fourier transform of Eq. (K.4), multiplying $\tilde{a}(\omega)$ with its complex conjugate, and using that the power spectrum of unit white noise is unity. We find

$$S_a(\omega) = \frac{2c_2 a^*}{c_2^2 + \omega^2}. \tag{K.5}$$

The power spectrum of the readout $\mathrm{B_T}$ is equivalent to the sum over all individual readout species' (cross-)power spectra,

$$S_{b_T}(\omega) = \sum_{i=1}^{N}\sum_{j=1}^{N} S_{b_i b_j}(\omega). \tag{K.6}$$

To obtain $S_{b_ib_j}(\omega)$ for all $i$ and $j$ it is most insightful to express the readout dynamics as an N-dimensional Ornstein-Uhlenbeck process

$$\frac{\mathrm{d}\delta b}{\mathrm{d}t} = G\delta a(t) + J\delta b(t) + B\xi(t), \tag{K.7}$$

with $\delta b = (b_1, \ldots, b_N)^T$, the $N \times 1$ gain matrix $G = (c_3, 0, \ldots, 0)^T$, the $N \times N$ network Jacobian

$$J = \begin{pmatrix} -\mu & 0 & 0 & \ldots & 0 & 0 \\ \mu & -\mu & 0 & \ldots & 0 & 0 \\ 0 & \mu & -\mu & \ldots & 0 & 0 \\ \vdots & \vdots & \vdots & \ddots & \vdots & \vdots \\ 0 & 0 & 0 & \ldots & -\mu & 0 \\ 0 & 0 & 0 & \ldots & \mu & -\mu \end{pmatrix}, \tag{K.8}$$

and the $N \times (N+1)$ matrix of noise strengths

$$B = \begin{pmatrix} \sqrt{c_3 a^*} & \sqrt{\mu b^*} & 0 & \ldots & 0 & 0 \\ 0 & \sqrt{\mu b^*} & \sqrt{\mu b^*} & \ldots & 0 & 0 \\ 0 & 0 & \sqrt{\mu b^*} & \ldots & 0 & 0 \\ \vdots & \vdots & \vdots & \ddots & \vdots & \vdots \\ 0 & 0 & 0 & \ldots & \sqrt{\mu b^*} & \sqrt{\mu b^*} \end{pmatrix}, \tag{K.9}$$

where $b^* = b_i^* = c_3 a^*/\mu$ is the mean concentration of each readout species. Note that $N+1$ is the number of reactions involving the readout species, and $B$ gives the noise strength associated with each reaction. The length $N+1$ unit white noise vector $\xi(t)$ in Eq. (K.7) describes the fluctuations induced by each reaction. Because the birth and death reactions of the signal are independent of the synthesis and decay reactions of the readout states, the power spectrum of each readout state obeys the spectral addition rule [22]. The matrix of all readout power spectra therefore has the following form

$$\mathbb{S}(\omega) = |\mathbb{K}(\omega)|^2 S_a(\omega) + |\mathbb{N}(\omega)|^2, \tag{K.10}$$

where

$$\mathbb{K}(\omega) = (i\omega\mathbb{I}_N - J)^{-1}G \tag{K.11}$$

defines all frequency dependent gains, and

$$\mathbb{N}(\omega) = (i\omega\mathbb{I}_N - J)^{-1}B \tag{K.12}$$

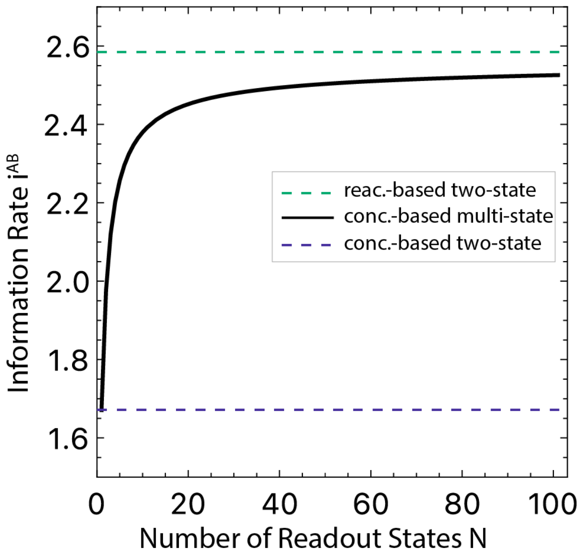


Figure 2: The state-based path mutual information rate of a simple linear network (Eqs. (K.1) and (K.2)) with $N$ readout states approaches the reaction-based path mutual information rate of the same network with a single readout state. The upper dashed line is the reaction-based path mutual information rate of motif a of the main text, and the lower dashed line is the state-based path mutual information rate of motif a of the main text (see Table 1). Parameters are set to $c_2 = 1$, $c_3 = 10$, $\mu = Nc_3$.

defines all frequency dependent noise terms of the individual readout states. The (cross-)power spectra $S_{b_i b_j}(\omega)$ between readout state $i$ and state $j$, which are required to compute the full power spectrum $S_{b_T}(\omega)$ (Eq. (K.6)), are given by the $(i,j)^{\text{th}}$ entry of the matrix of all readout power spectra (Eq. (K.10))

$$S_{b_i b_j}(\omega) = \mathbb{S}_{(i,j)}(\omega) = |\mathbb{K}(\omega)|^2_{(i,j)} S_a(\omega) + |\mathbb{N}(\omega)|^2_{(i,j)}. \tag{K.13}$$

Substitution of Eq. (K.13) in Eq. (K.6) yields

$$S_{b_T}(\omega) = |K_{b_T}(\omega)|^2 S_a(\omega) + |N_{b_T}(\omega)|^2, \tag{K.14}$$

with the frequency dependent gain from $a(t)$ to $b_T(t)$,

$$|K_{b_T}(\omega)|^2 = \sum_{i=1}^{N}\sum_{j=1}^{N} |\mathbb{K}(\omega)|^2_{(i,j)} = c_3^2 \sum_{i=1}^{N}\sum_{j=1}^{N} \frac{\mu^{i+j-2}}{(\mu+i\omega)^i(\mu-i\omega)^j}. \tag{K.15}$$

and the frequency dependent noise in $b_T(t)$,

$$|N_{b_T}(\omega)|^2 = \sum_{i=1}^{N}\sum_{j=1}^{N} |\mathbb{N}(\omega)|^2_{(i,j)} = c_3 a^* \sum_{i=1}^{N} (N-i+1)\mu^{i-2}\left(\frac{1}{(\mu+i\omega)^i} + \frac{1}{(\mu-i\omega)^i}\right), \tag{K.16}$$

where we used that $\mu b^* = c_3 a^*$ to compute the elements of $|\mathbb{N}(\omega)|^2$.

Finally, we rearrange the expression for the path mutual information rate (Eq. K.3), using Eq. (K.14) and the cross-spectrum between $a(t)$ and $b_T(t)$ given by $|S_{ab_T}(\omega)|^2 = |K_{b_T}(\omega)|^2 |S_a(\omega)|^2$ to obtain,

$$i_{\text{sb}}^{ab_T} = \frac{1}{4\pi}\int_{-\infty}^{\infty} d\omega \log\left(1 + \frac{|K_{b_T}(\omega)|^2}{|N_{b_T}(\omega)|^2} S_a(\omega)\right), \tag{K.17}$$

as also shown in [12, 21]. We now compute the state-based information rate of the multi-state motif shown in (K.1) over the number of readout states $N$ by substituting Eqns. (K.5), (K.15) and (K.16) in Eq. (K.17) and integrating numerically for every $N$. Figure 2 shows that the resulting information rate indeed starts from the state-based path mutual information rate of motif a at $N = 1$ (main text Table 1), and approaches the reaction-based information rate of motif a as $N$ increases. Notably, the path mutual information rate rises strongly with the first few additional states.

## References


[1] N. G. Van Kampen, *Stochastic processes in physics and chemistry*, vol. 1. Elsevier, 1992.

[2] D. T. Gillespie, "The chemical Langevin equation," *The Journal of Chemical Physics*, vol. 113, pp. 297–306, July 2000.

[3] E. W. J. Wallace, "A simplified derivation of the linear noise approximation," *arXiv preprint arXiv:1004.4280*, 2010.

[4] P. Thomas and R. Grima, "Approximate probability distributions of the master equation," *Phys. Rev. E*, vol. 92, p. 012120, Jul 2015.

[5] R. S. Liptser and A. N. Shiriaev, *Statistics of random processes: General theory*, vol. 394. Springer, 1977.

[6] T. Kailath, "The innovations approach to detection and estimation theory," *Proceedings of the IEEE*, vol. 58, no. 5, pp. 680–695, 1970.

[7] R. L. Dobrushin and D. Surgailis, "On the innovation problem for gaussian markov random fields," *Wahrscheinlichkeitstheorie verw. Gebiete*, vol. 49, pp. 275–291, 1979.

[8] R. E. Spinney, M. Prokopenko, and J. T. Lizier, "Transfer entropy in continuous time, with applications to jump and neural spiking processes," *Physical Review E*, vol. 95, p. 032319, Mar. 2017. arXiv:1610.08192 [cs].

[9] T. T. Kadota, M. Zakai, and J. Ziv, "Mutual Information of the White Gaussian Channel With and Without Feedback," in *IEEE Transactions on Information Theory*, vol. 17, pp. 368–371, 1971.

[10] M. Hitsuda, "Mutual information in gaussian channels," *Journal of Multivariate Analysis*, vol. 4, no. 1, pp. 66–73, 1974.

[11] T. E. Duncan, "On the calculation of mutual information," *SIAM Journal on Applied Mathematics*, vol. 19, no. 1, pp. 215–220, 1970.

[12] F. Tostevin and P. R. ten Wolde, "Mutual information between input and output trajectories of biochemical networks," *Phys. Rev. Lett.*, vol. 102, p. 218101, May 2009.

[13] F. Tostevin and P. R. ten Wolde, "Mutual information in time-varying biochemical systems," *Phys. Rev. E*, vol. 81, p. 061917, Jun 2010.

[14] R. E. Kálmán and R. S. Bucy, "New results in linear filtering and prediction theory," *Journal of Basic Engineering*, vol. 83, pp. 95–108, 1961.

[15] A. Bain and D. Crisan, *Fundamentals of stochastic filtering*, vol. 3. Springer, 2009.

[16] A. Kutschireiter, S. C. Surace, and J.-P. Pfister, "The hitchhiker's guide to nonlinear filtering," *Journal of Mathematical Psychology*, vol. 94, p. 102307, 2020.

[17] "6 nonlinear filtering theory," in *Stochastic Processes and Filtering Theory*, vol. 64 of *Mathematics in Science and Engineering*, pp. 162–193, Elsevier, 1970.

[18] G. Malaguti and P. R. ten Wolde, "Receptor time integration via discrete sampling," *Phys. Rev. E*, vol. 105, p. 054406, May 2022.

[19] P. R. ten Wolde, N. B. Becker, T. E. Ouldridge, and A. Mugler, "Fundamental Limits to Cellular SensingPieter Rein ten Wolde, Nils B. Becker, Thomas E. Ouldridge & Andrew Mugler," *Journal of Statistical Physics*, vol. 162, pp. 1395–1424, Jan. 2016.

[20] R. G. Endres and N. S. Wingreen, "Maximum likelihood and the single receptor," *Phys. Rev. Lett.*, vol. 103, p. 158101, Oct 2009.

[21] W. H. de Ronde, F. Tostevin, and P. R. ten Wolde, "Effect of feedback on the fidelity of information transmission of time-varying signals," *Phys. Rev. E*, vol. 82, p. 031914, Sep 2010.

[22] P. B. Warren, S. Tănase-Nicola, and P. R. Ten Wolde, "Exact results for noise power spectra in linear biochemical reaction networks," *Journal of Chemical Physics*, vol. 125, pp. 144904–144904, Oct. 2006.
